# Supplementary material for: Towards Generalizing to Unseen Domains with Few Labels
Source: arXiv:2403.11674 source file (2024-05-07)
Supplement: Supplementary file 1 [file X_suppl.tex]

\clearpage
\setcounter{page}{1}
\maketitlesupplementary

\section{Datasets Description}

\noindent\textbf{PACS:} PACS dataset consists of four domains: photo (1,670 images), art painting (2,048 images), cartoon (2,344 images)  and sketch (3,929 images), and seven classes: dog, elephant, giraffe, guitar, horse, house, and person.

\noindent\textbf{OfficeHome:} The OfficeHome dataset also consists of four domains: art, clipart, product, and the real world with 65 different classes whose total number of images adds up to around 15,500. 

\noindent\textbf{Digits-DG:} The Digits-DG dataset consists of four domains: MNIST, MNIST-M, SVHN, and SYN, and 10 classes from 0 to 9. MNIST comprises hand-written digits, MNIST-M is a variant of MNIST with a blended background, SVHN has street-view house numbers and SYN consists of synthetic digits. 

\noindent\textbf{VLCS:} VLCS dataset consists of four domains: Caltech, Labelme, Pascal, and Sun with 5 classes: bird, car, chair, dog, and person

\noindent\textbf{Terra Incognita:} This dataset contains images belonging to four domains collected from different locations namely locations 38, 43,46 and 100 with 10 classes: bird, bobcat, cat, coyote, dog, empty, opossum, rabbit, raccoon, and squirrel. 

Figure~\ref{fig:data} displays randomly selected samples from each dataset. 

\begin{figure*}[!htp] % "[t!]" placement specifier just for this example
\begin{subfigure}{0.48\textwidth}
\includegraphics[width=\linewidth]{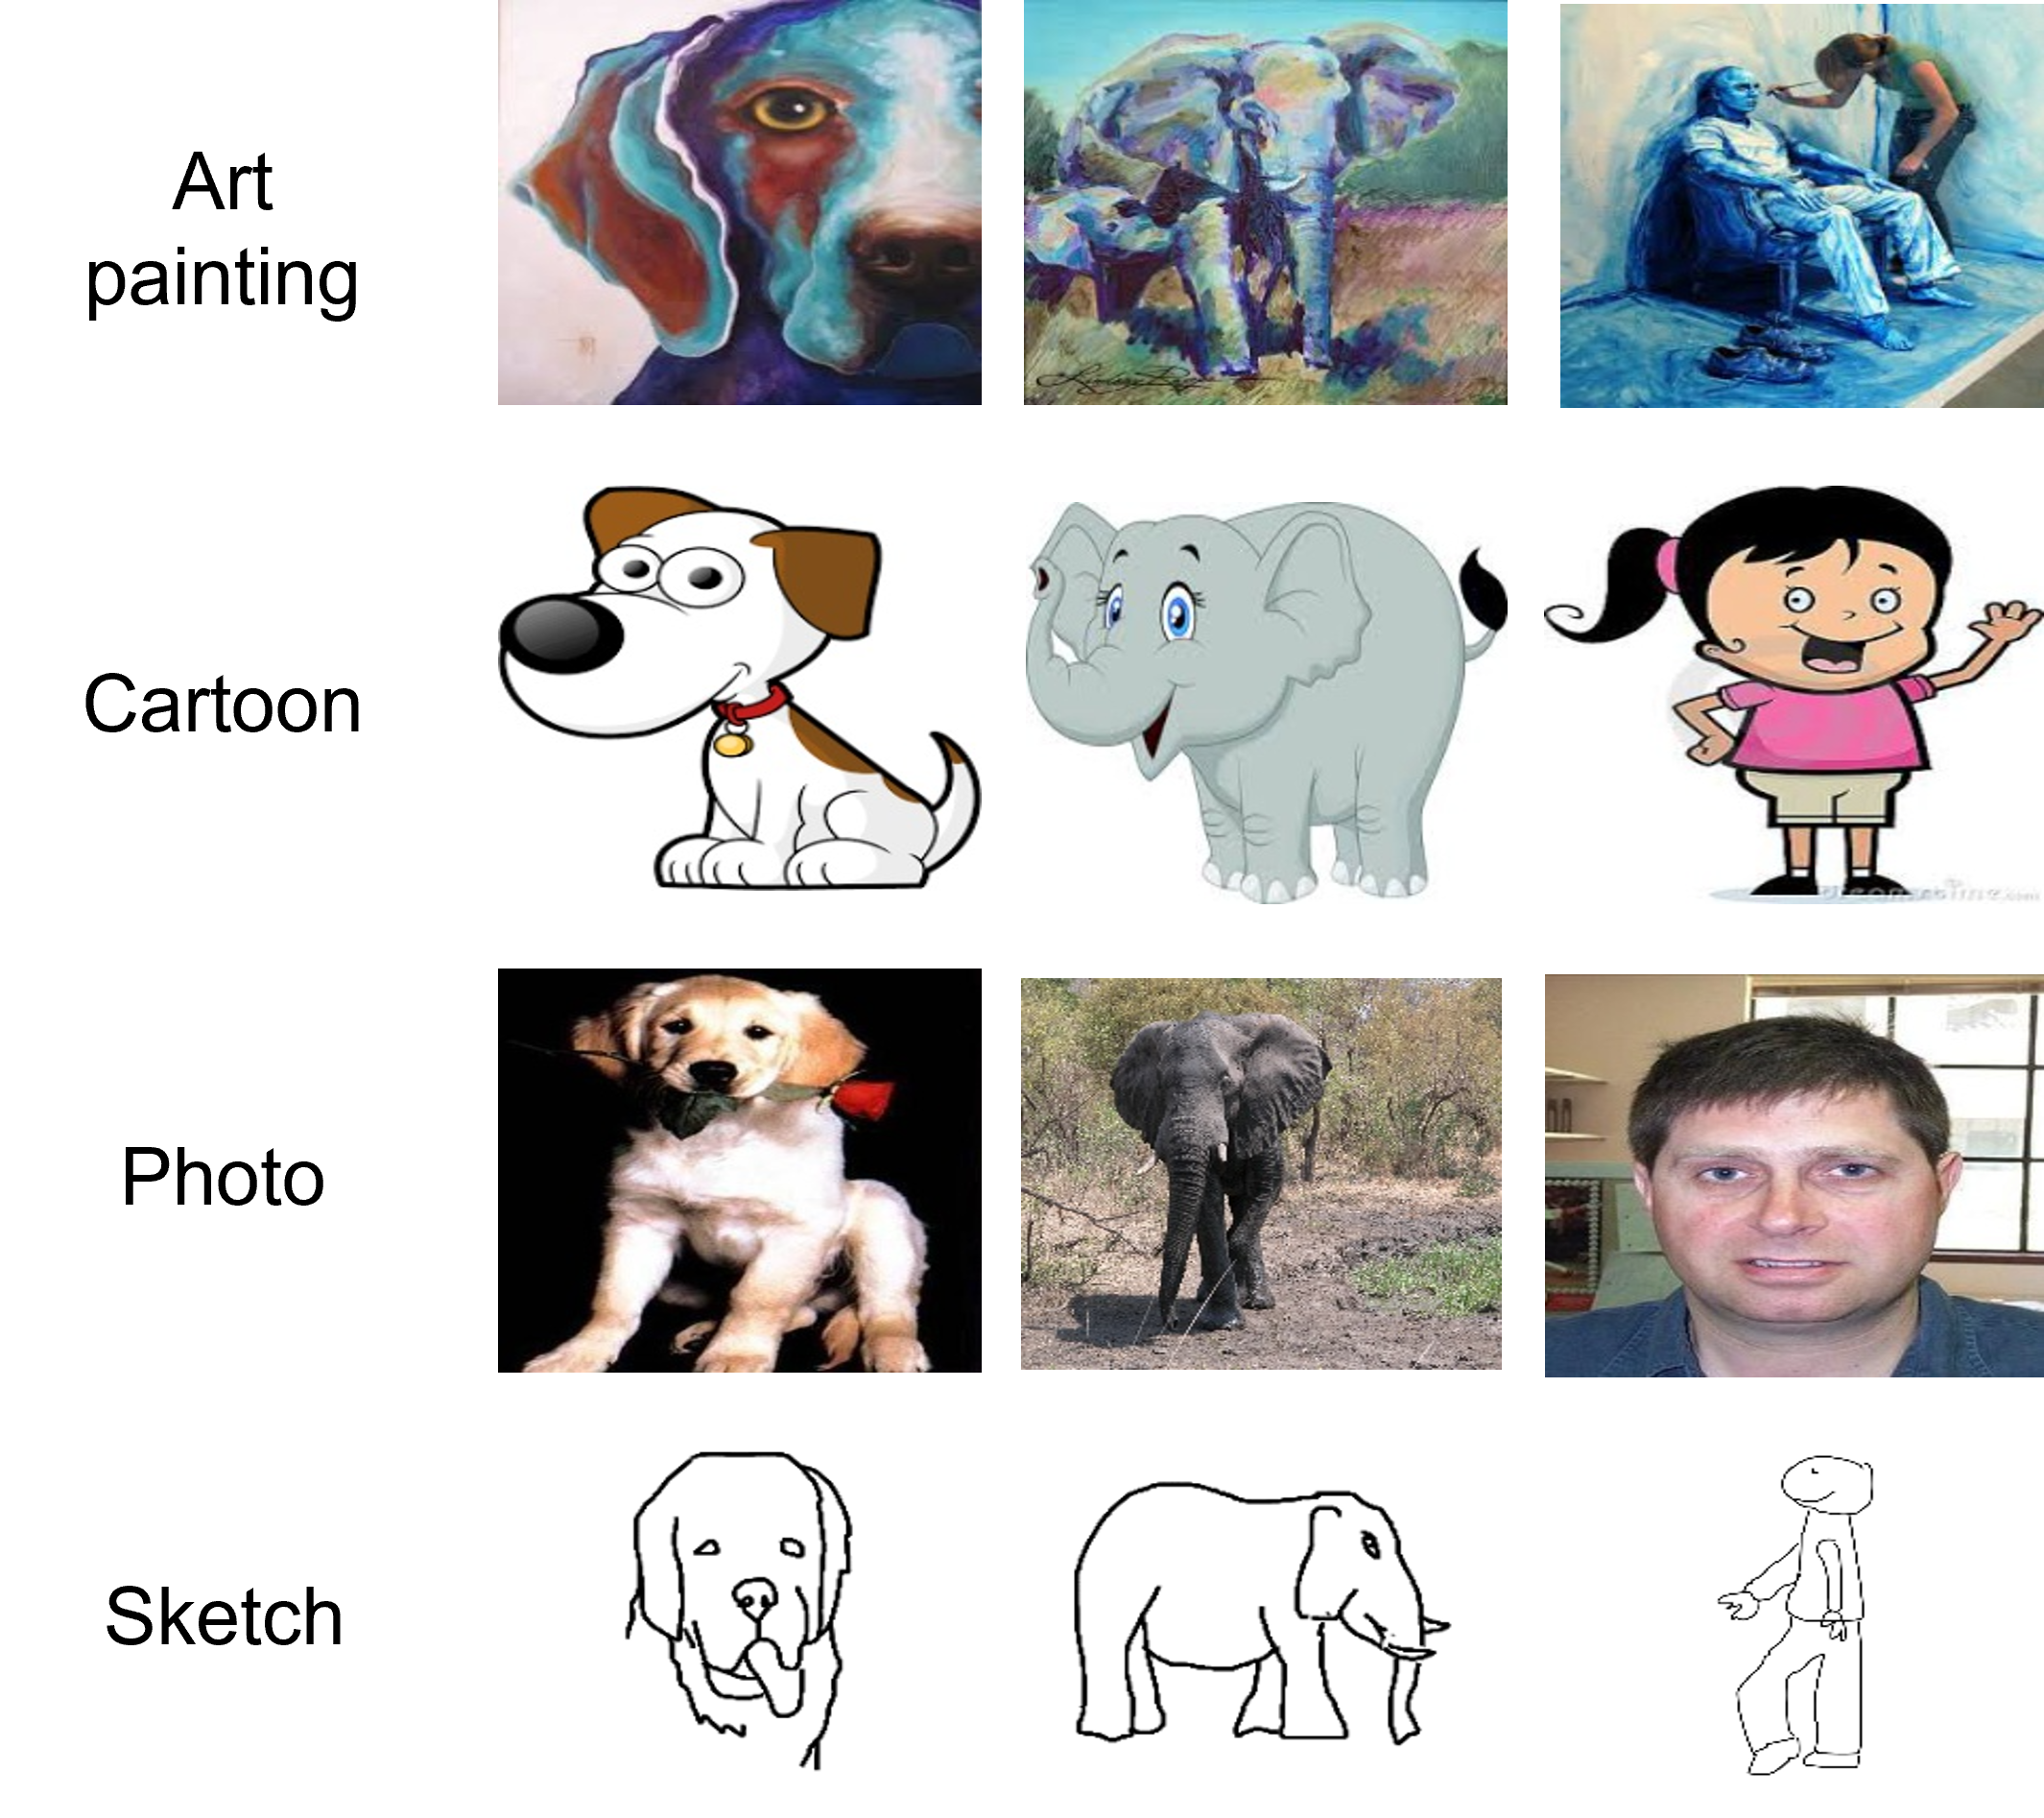}
\caption{PACS} \label{fig:a}
\end{subfigure}\hspace*{\fill}
\begin{subfigure}{0.48\textwidth}
\includegraphics[width=\linewidth]{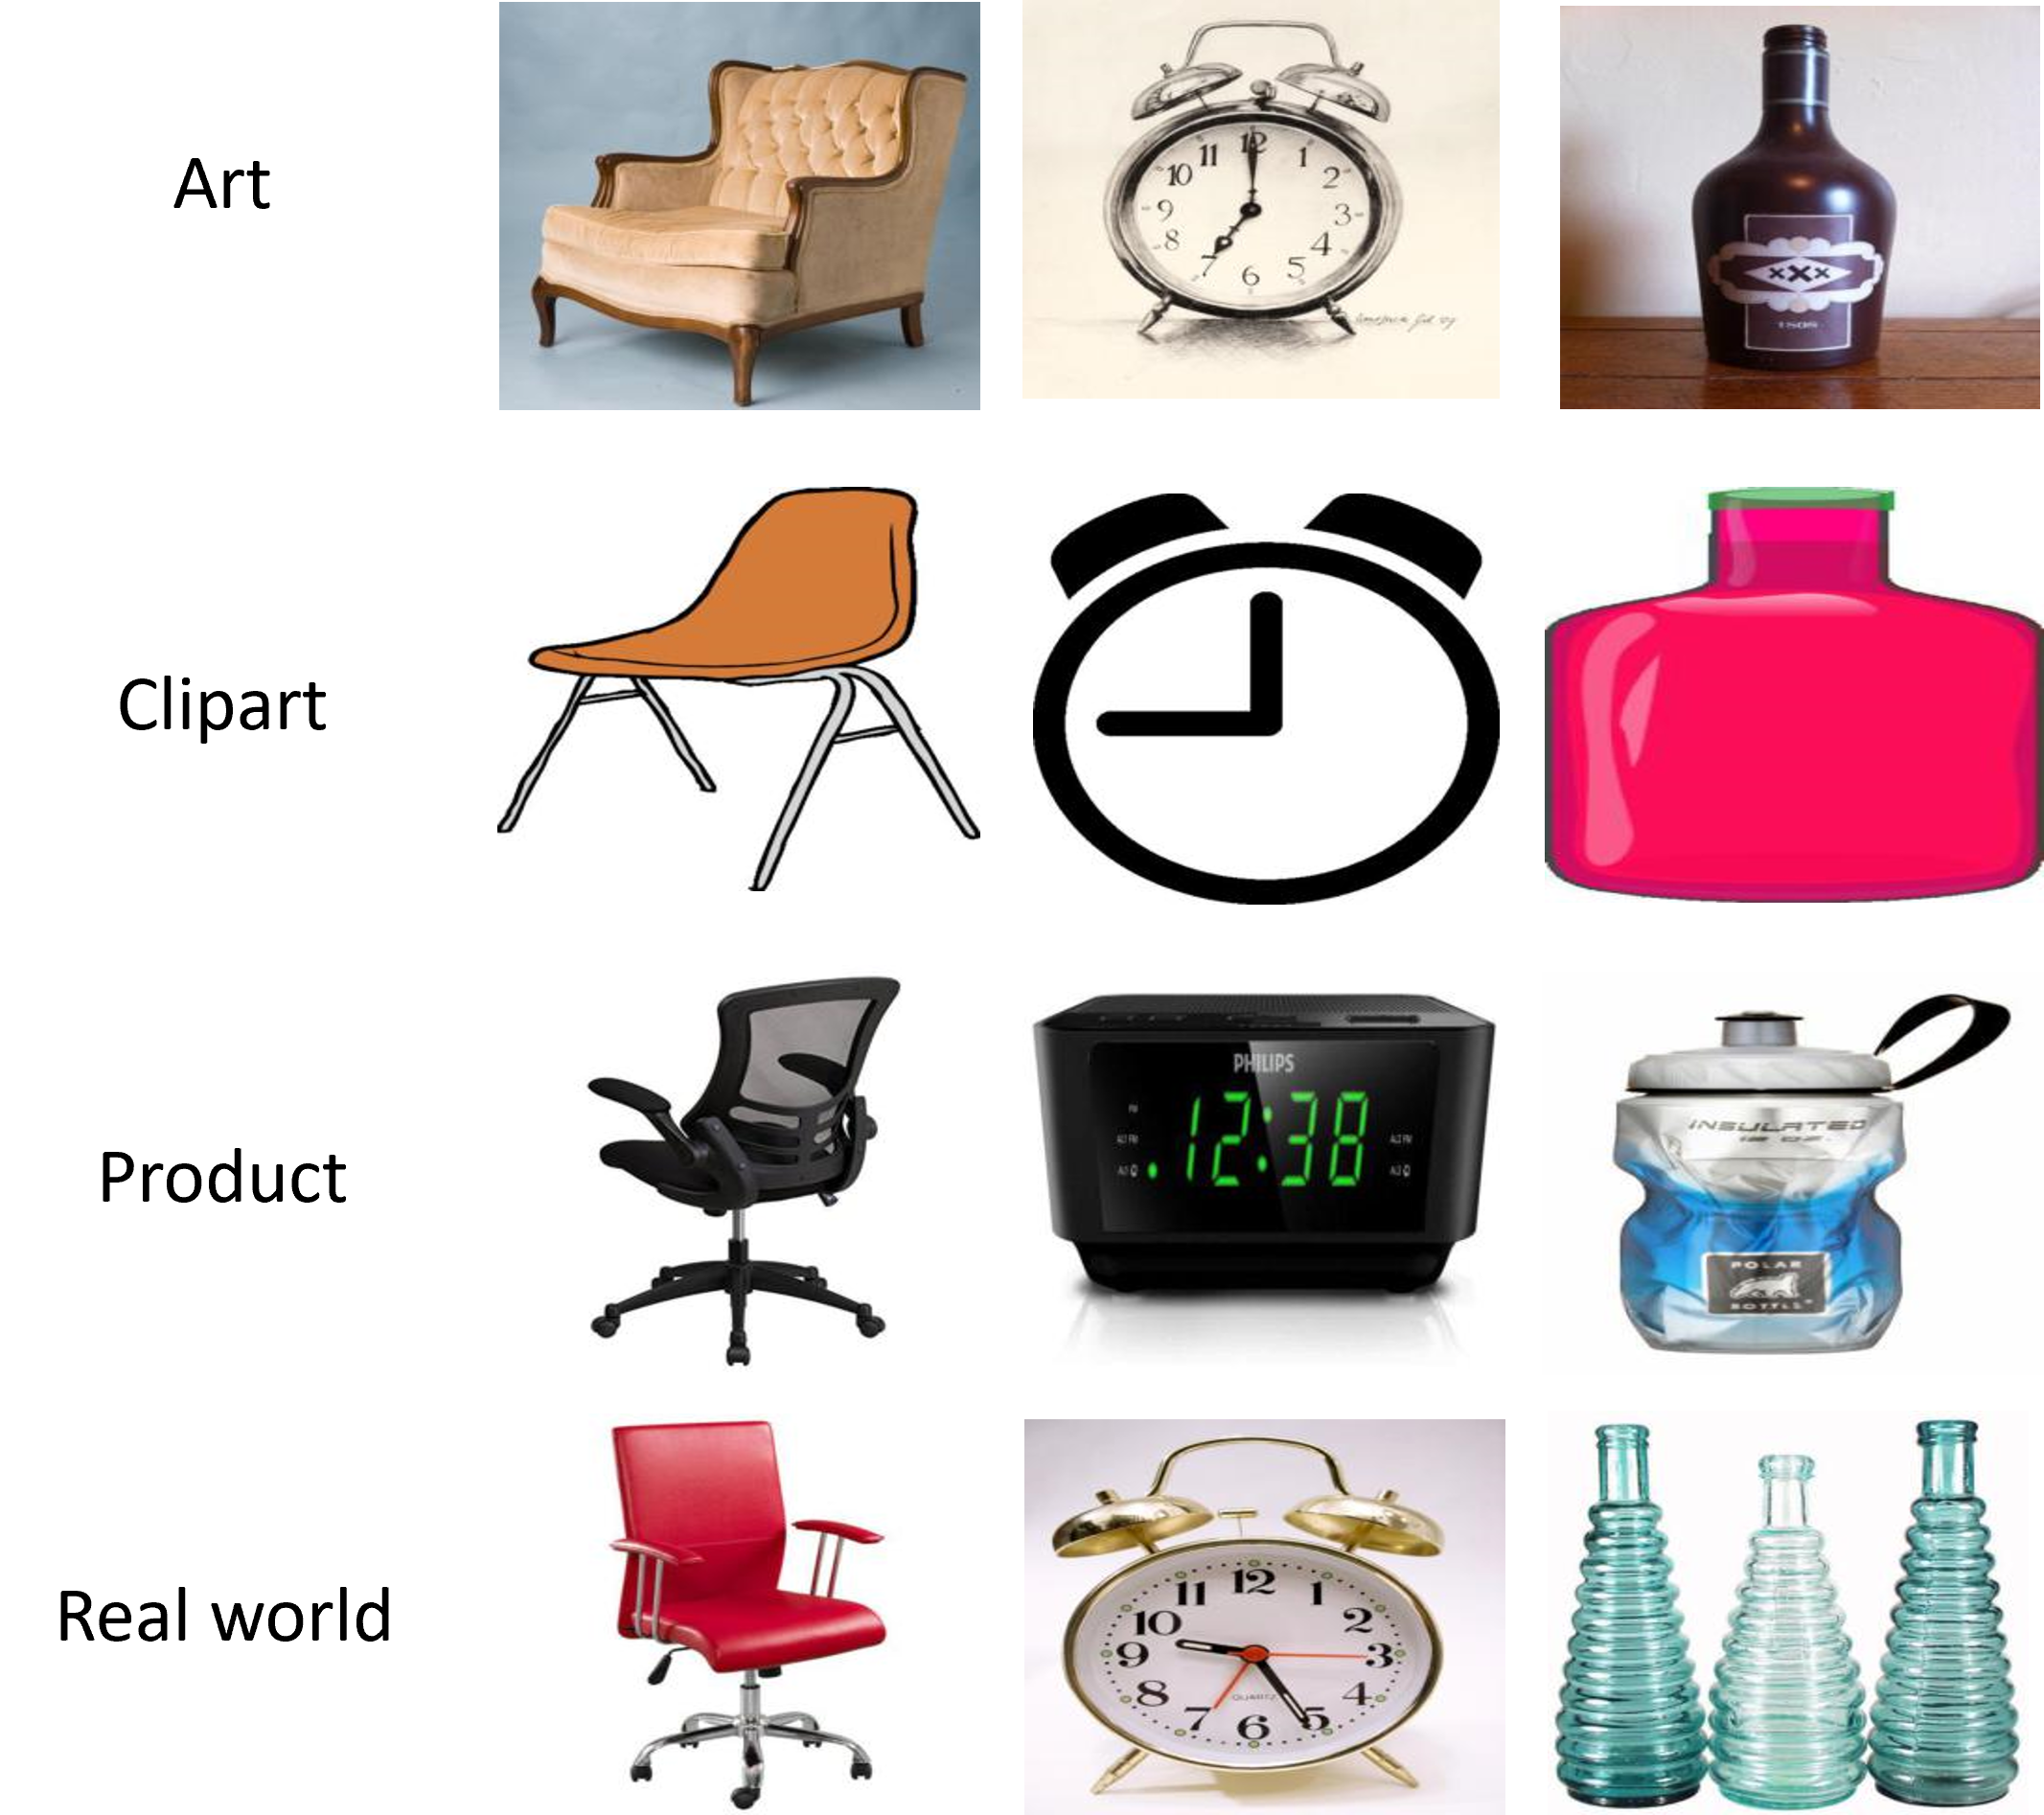}
\caption{OfficeHome} \label{fig:b}
\end{subfigure}

\medskip
\begin{subfigure}{0.48\textwidth}
\includegraphics[width=\linewidth]{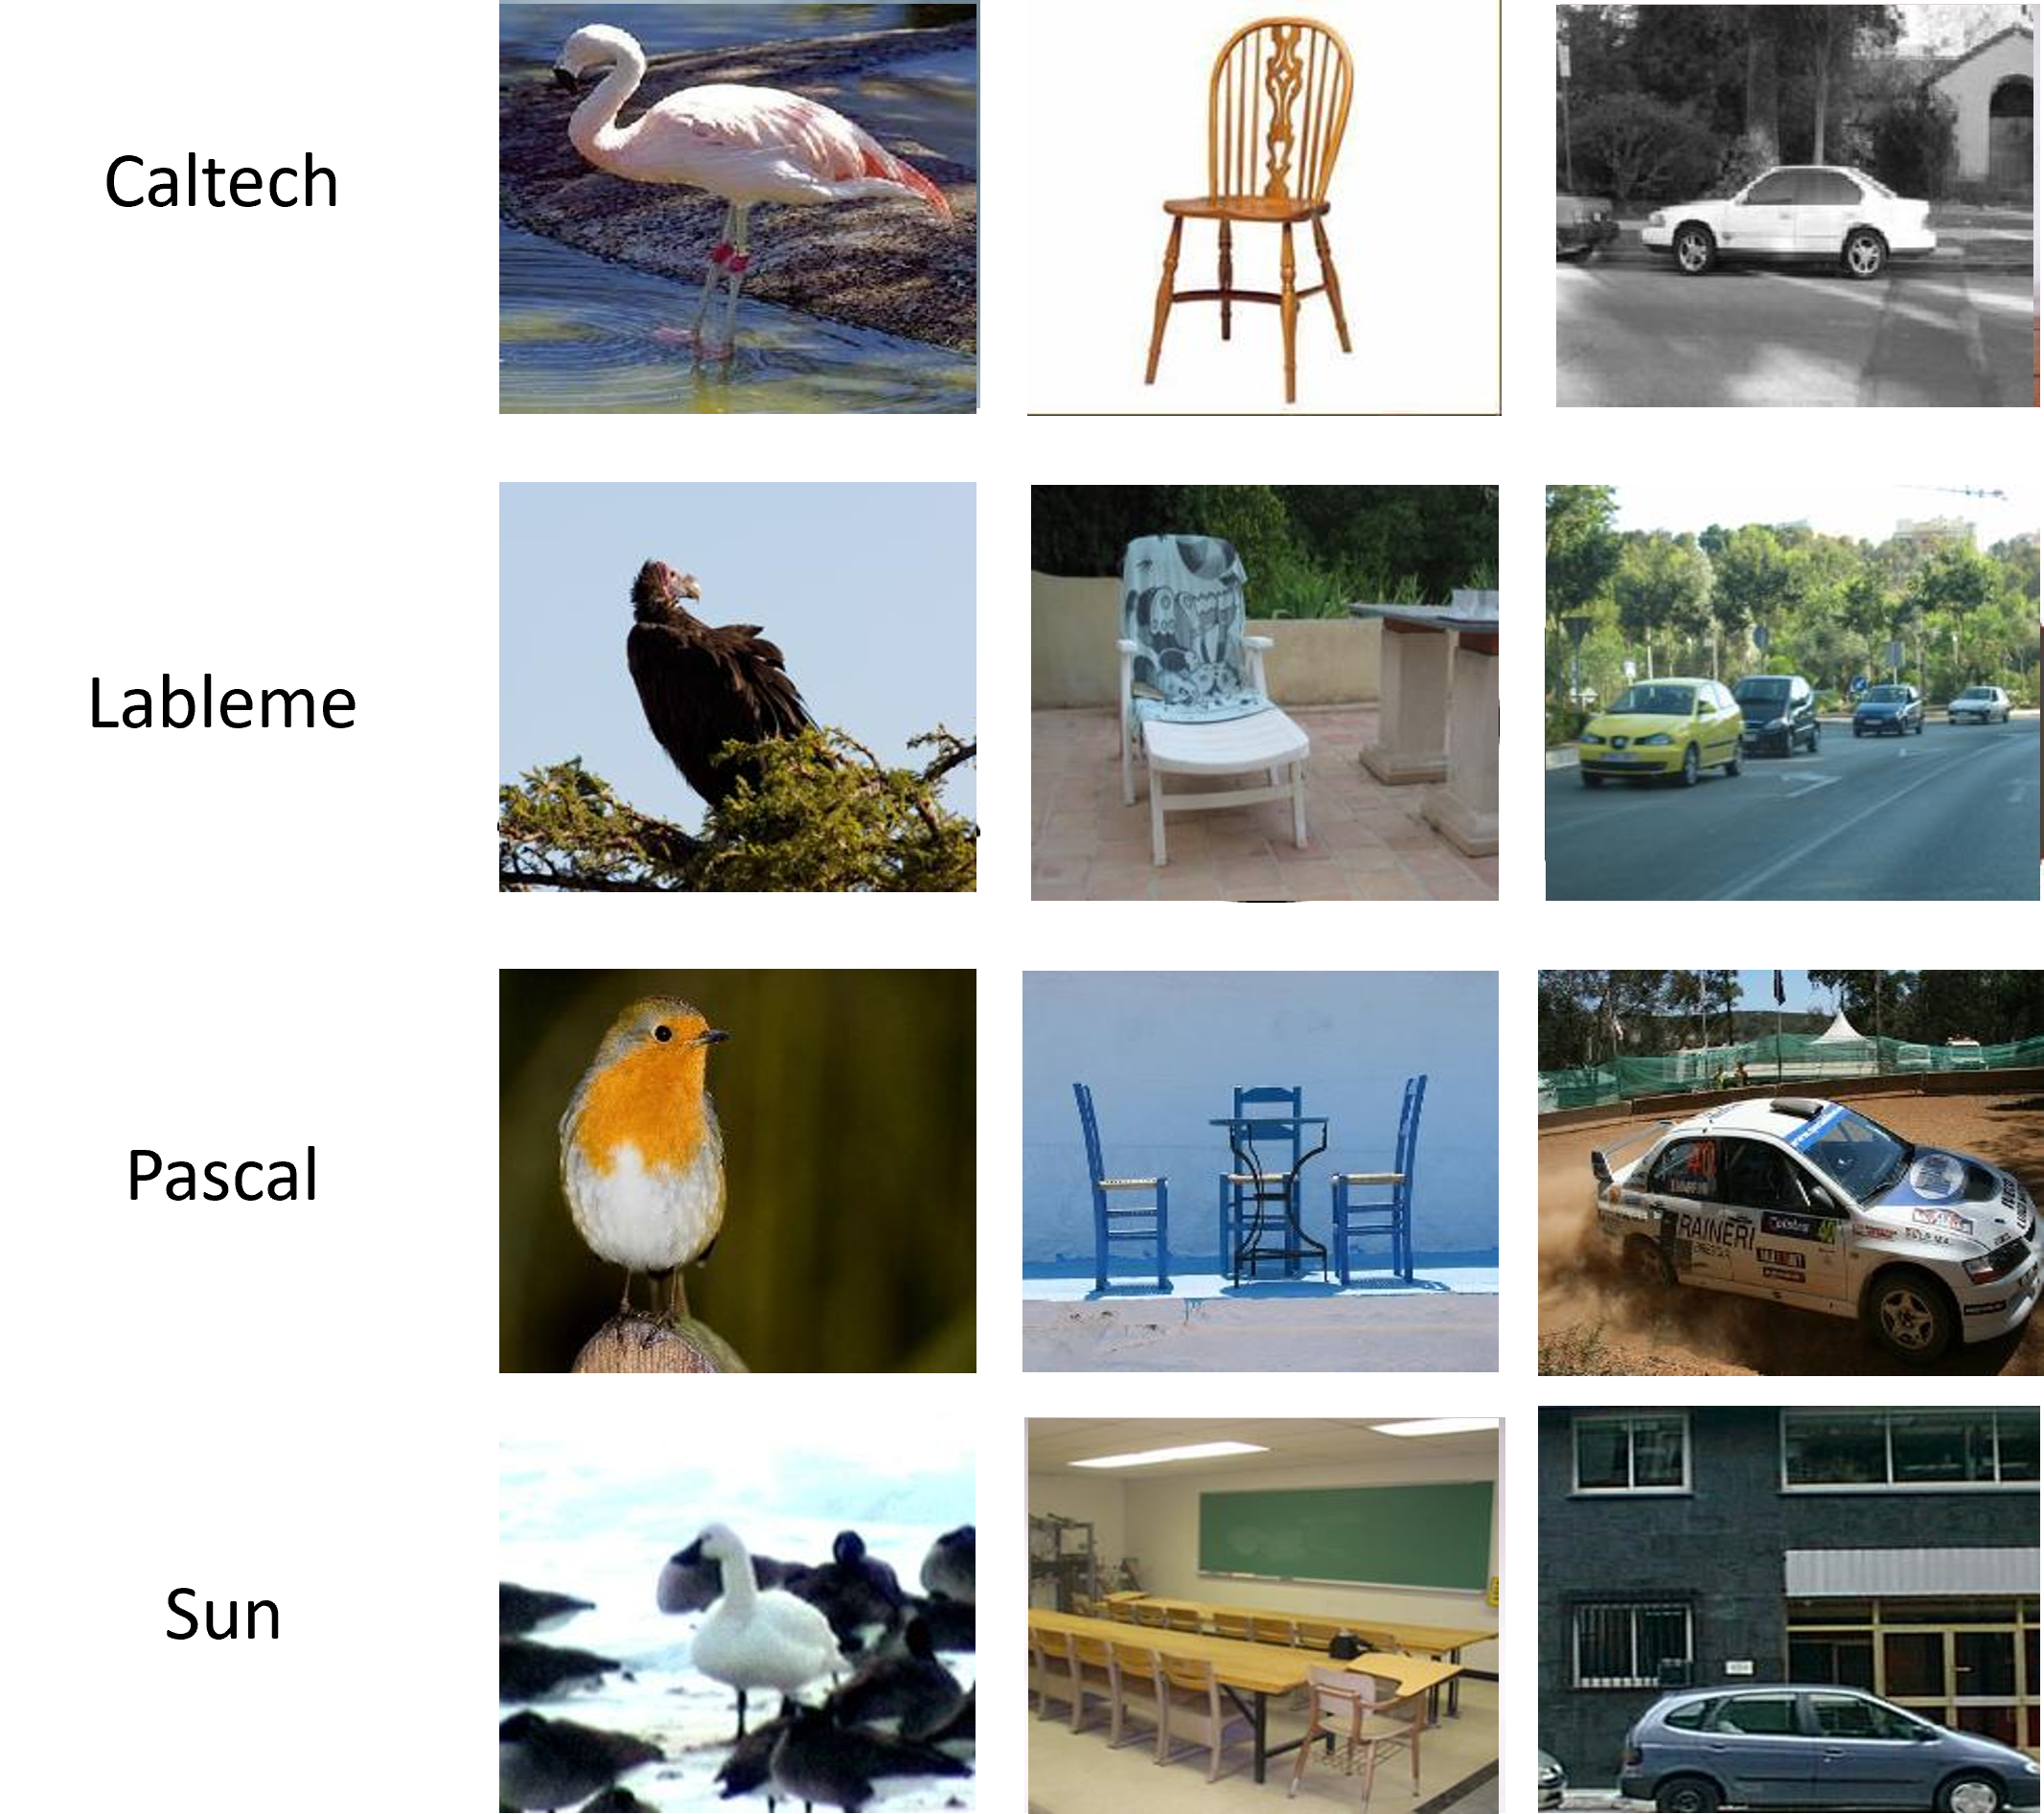}
\caption{VLCS} \label{fig:c}
\end{subfigure}\hspace*{\fill}
\begin{subfigure}{0.48\textwidth}
\includegraphics[width=\linewidth]{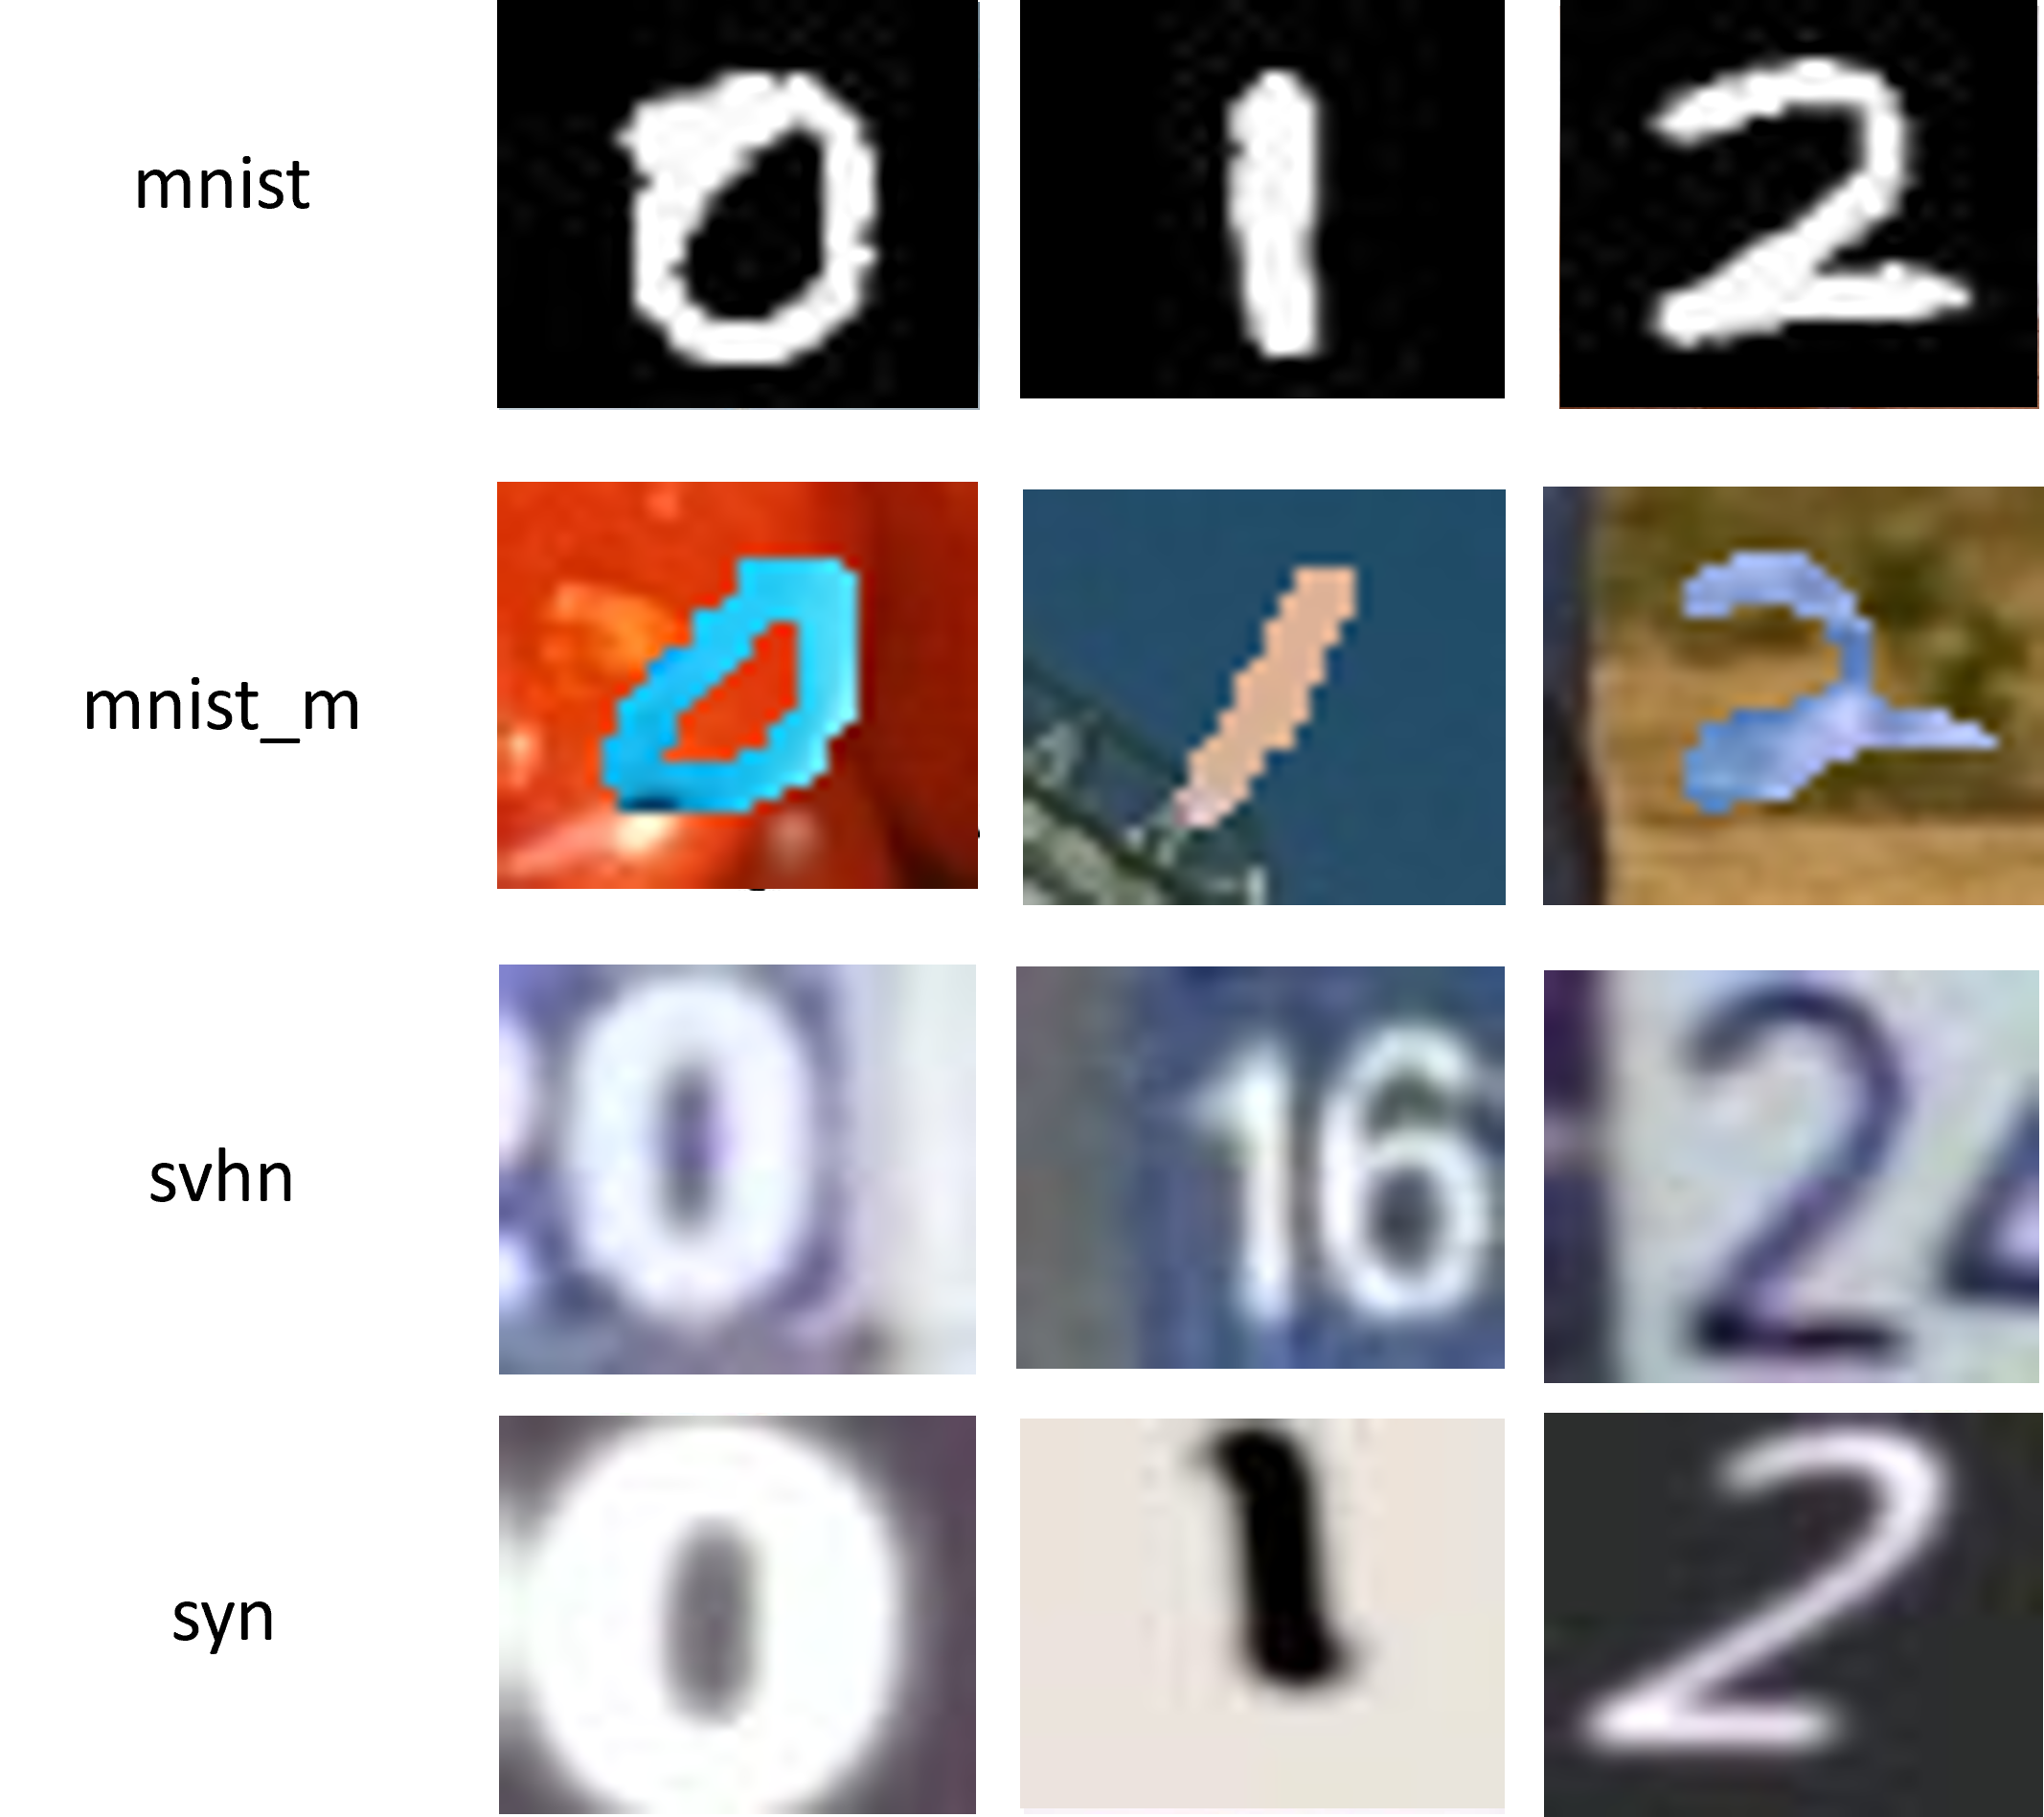}
\caption{Digits-DG} \label{fig:d}
\end{subfigure}

\medskip
\begin{subfigure}{0.98\textwidth}
\centering
\includegraphics[width=0.5\linewidth]{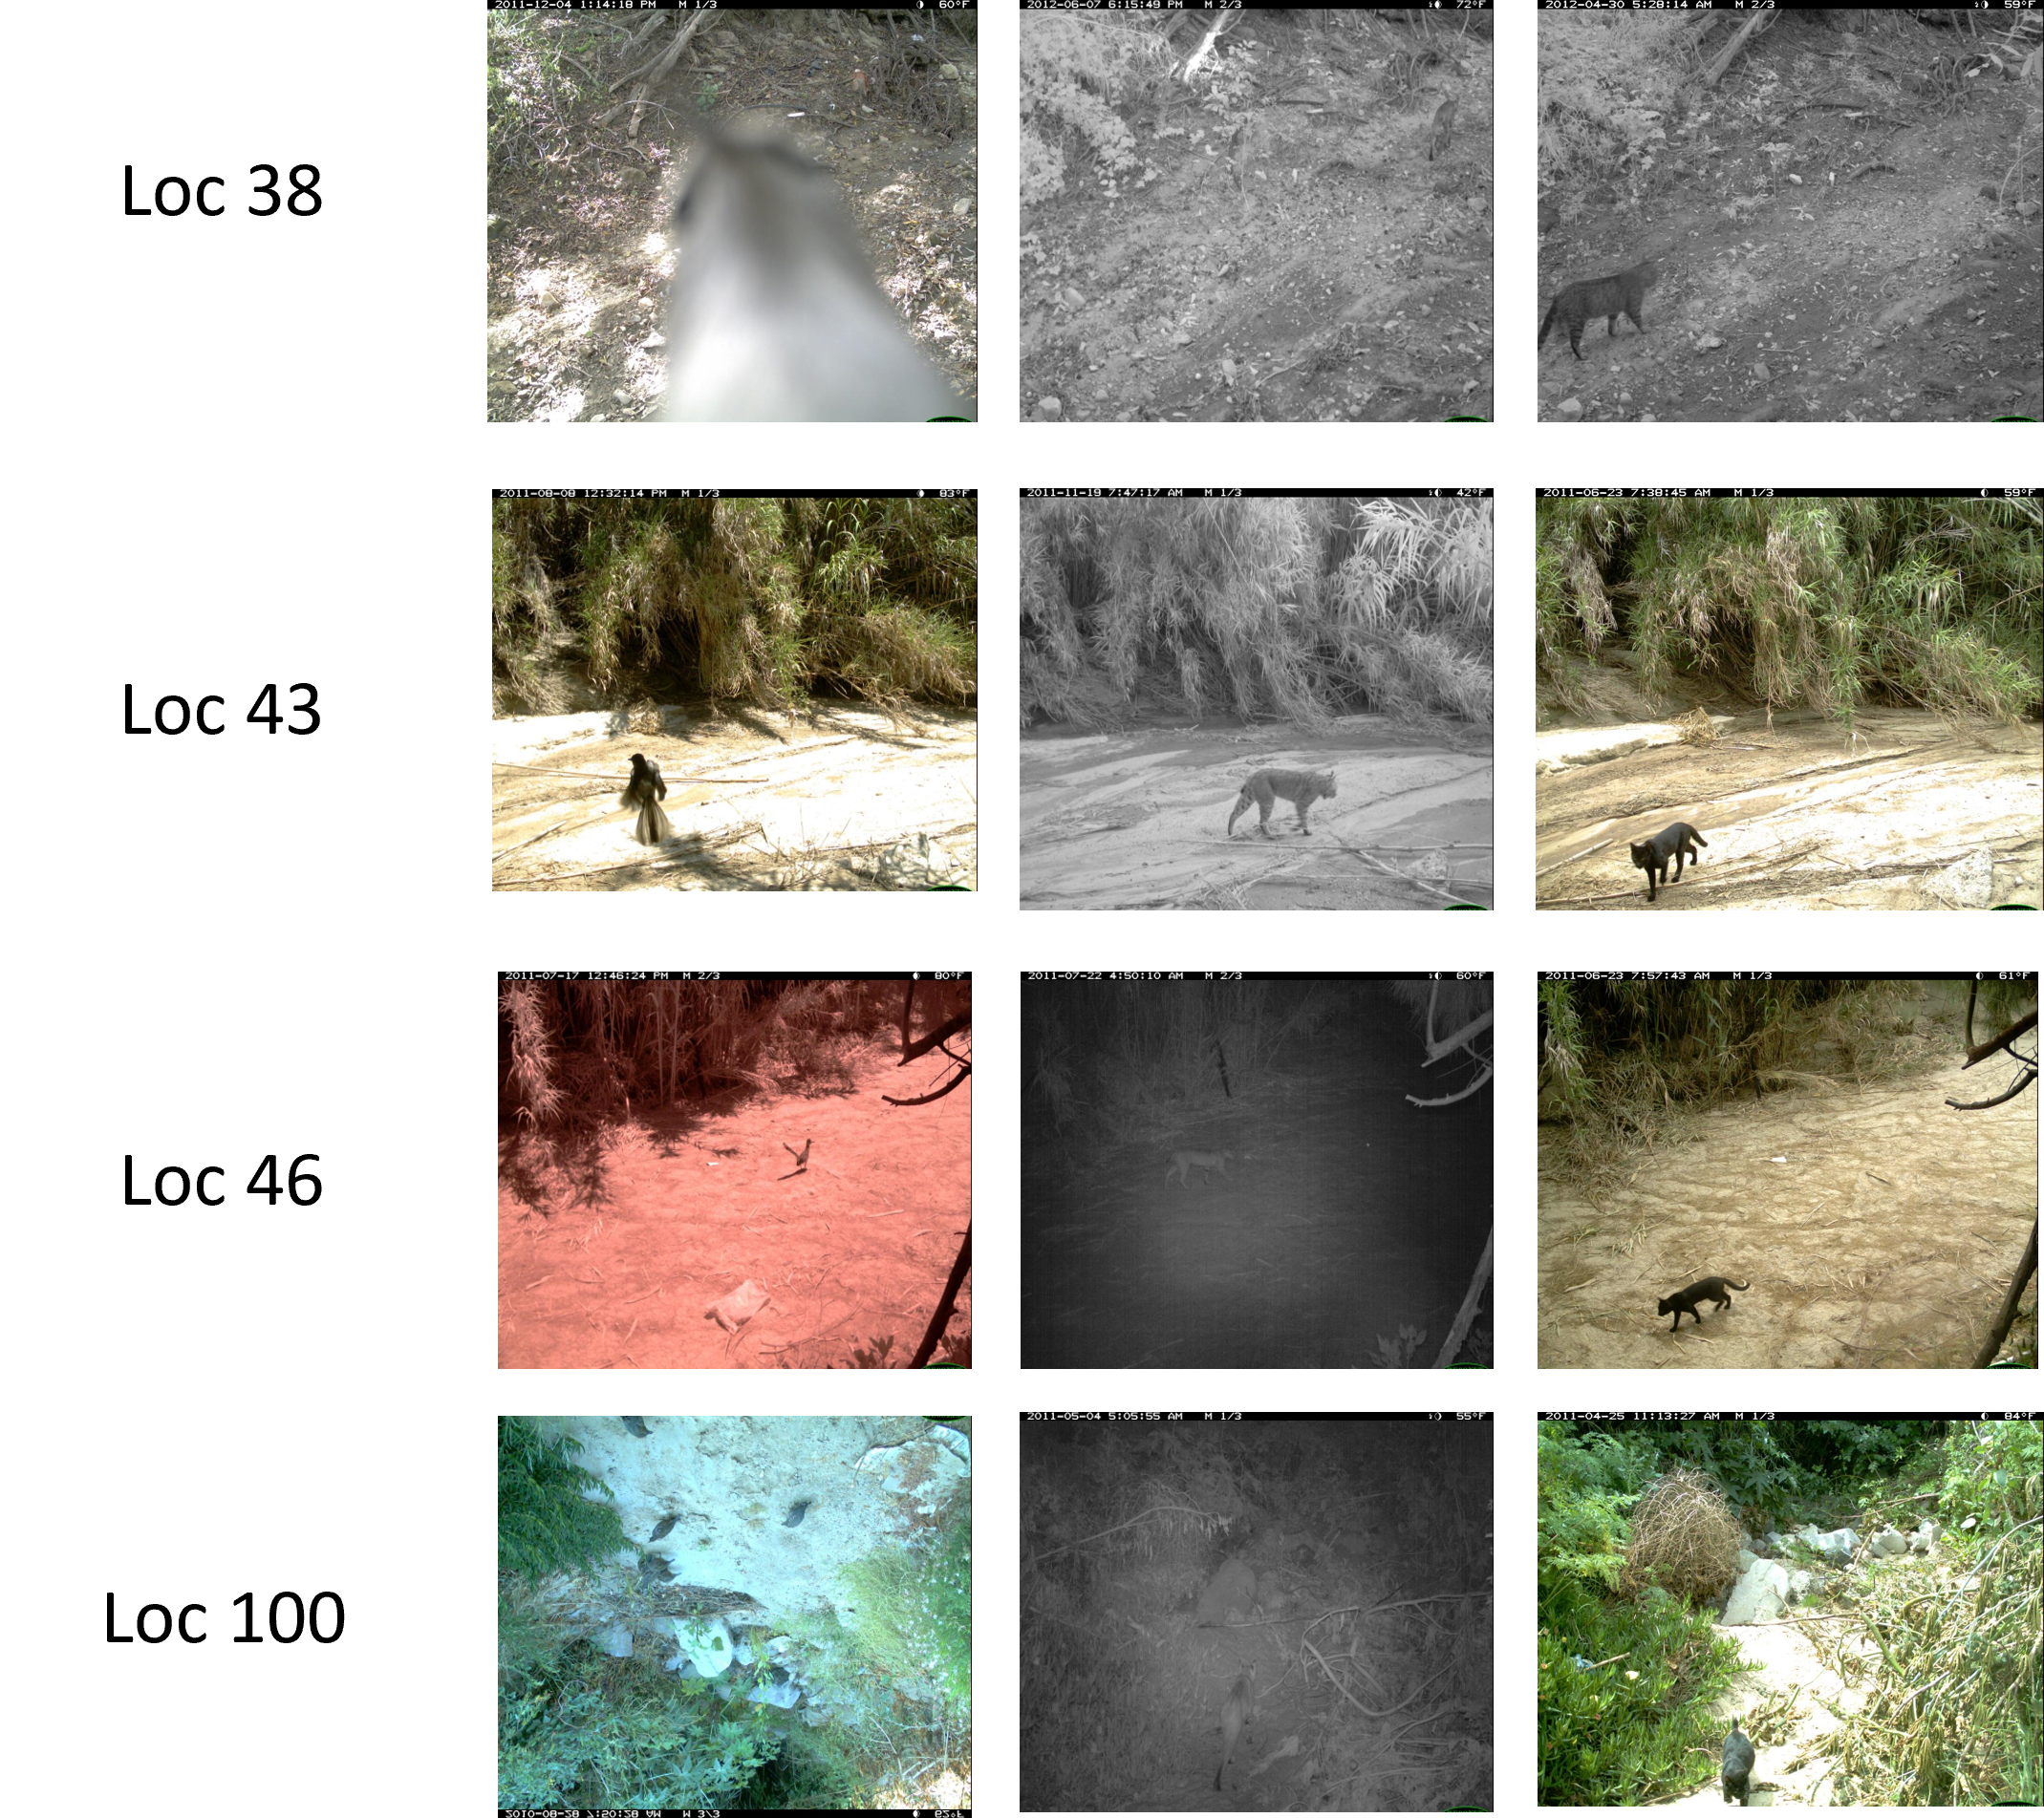}
\caption{Terra Incognita} \label{fig:e}
\end{subfigure}\hspace*{\fill}
% \begin{subfigure}{0.48\textwidth}
% \includegraphics[width=\linewidth]{pic6.pdf}
% \caption{Sixth subfigure} \label{fig:f}
% \end{subfigure}

\caption{Example images from different DG datasets used in our experiments.} \label{fig:data}
\end{figure*}

\section{Comparison with DG baselines}

We choose ERM \cite{vapnik1999nature}, MixUp \cite{zhang2018mixup}, GroupDRO \cite{sagawa2019distributionally}, CrossGrad \cite{shankar2018generalizing}, DAELDG \cite{DBLP:journals/corr/abs-2003-07325}
, DDAIG \cite{zhou2020deep} and DomainMix \cite{sun2022dynamic} as DG baselines to compare our method on PACS, OfficeHome, Digits-DG, VLCS and TerraIncognita datasets under both 5 labels (see Tab.~\ref{tab:5_labels_DG}) and 10 labels (see Tab.~\ref{tab:10_labels_DG}) settings.

\section{Additional class similarity matrices}

To show the effectiveness of our algorithm, we show cosine similarity between the class means on PACS dataset in the main manuscript. In this supplementary, we also show this on Digits-DG dataset (see Fig.~\ref{fig:Digits_sim}). We see that, our losses encourage orthogonality among features with different class labels, and hence better discrimination in the feature space under different domain shifts and limited labels. Especially in Mnist-m, and Syn domains the similarities are notably higher compared to the Fixmatch baseline.

\begin{table*}[!ht]
\centering
\setlength{\tabcolsep}{15pt}

\begin{tabular}{lccccc}
\toprule
Model               & PACS  & OH & VLCS & DigitsDG & TerraInc. \\
\midrule
ERM                 & $51.2\pm3.0$  & $51.7\pm0.6$ & $67.2\pm1.8$      & $22.7\pm1.0$      & $22.9\pm3.0$   \\ 
MixUp & $ 45.3\pm 3.8$ & 52.7 $\pm$0.6 & $69.9\pm$ 1.3& $21.7\pm$ 1.9& 21.0$\pm$2.9 \\
GroupDRO& $ 48.2\pm 3.6$ & 53.8$\pm0.6$ & $69.8\pm1.2$ &$23.1 \pm$1
9& $22.4\pm3.1$ \\
CrossGrad& $ 50.6\pm 3.4$ & $51.6\pm0.9$ & $68.1\pm1.6$ & $22.8\pm0.4$ & $21.4\pm2.3$ \\
DAELDG& $ 42.7\pm 2.7$ & $47.3\pm0.6$ & $61.7\pm1.9$ & $22.3\pm1.0$ & $25.0\pm3.0$ \\
DDAIG&  $ 50.5\pm 3.0$ & $50.6\pm0.7$ & $65.2\pm2.2$ & $23.2\pm1.8$ & $31.7\pm3.1$ \\
DomainMix& $ 46.3\pm 3.5$ & $49.9\pm0.6$ & $68.3\pm0.7$ & $20.6\pm1.4$ & $22.9\pm0.9$ \\
\bottomrule
\end{tabular}
\caption{DG accuracy (\%) under SSDG settings (5 labels per class). Average over 5 independent seeds is reported. }
\vspace{-1em}
\label{tab:5_labels_DG}
\end{table*}

\begin{table*}[!ht]
\centering
\setlength{\tabcolsep}{15pt}

\begin{tabular}{lccccc}
\toprule
Model               & PACS  & OH & VLCS & DigitsDG & TerraInc. \\
\midrule
ERM  & $59.8\pm2.3$ & $56.7\pm0.8$ &$68.0\pm0.3$& $29.1\pm2.9$& $23.5\pm1.2$  \\ 
MixUp    & $58.5\pm2.2$ & $57.2\pm0.6$ & $69.6\pm1.0$ &$29.7\pm3.1$ &$24.8\pm3.3$ \\
GroupDRO    & $57.3\pm1.2$ &$57.8\pm0.4$ &$69.4\pm0.9$ &$31.5\pm2.5$ &$25.8\pm3.3$ \\
CrossGrad   &$59.7\pm1.5$ & $56.7\pm0.4$ & $67.9\pm0.6$ & $30.3\pm2.7$ & $22.6\pm0.9$\\
DAELDG      &$53.7\pm2.1$ &$54.8\pm0.3$ &$68.3\pm1.3$ &$28.6\pm1.5$ &$25.5\pm2.6$ \\
DDAIG       & $59.6\pm1.6$ &$55.1\pm0.1$ & $68.5\pm1.0$& $29.4\pm3.0$&$ 23.5\pm3.0$\\
DomainMix   & $58.0\pm1.9$& $55.4\pm0.4$& $69.5\pm0.8 $& $24.6\pm1.1$& $23.3\pm2.1$\\
\bottomrule
\end{tabular}
\caption{DG accuracy (\%) under SSDG settings (10 labels per class). Average over 5 independent seeds is reported. }
\vspace{-1em}
\label{tab:10_labels_DG}
\end{table*}

\begin{figure*}[!htp]
    \centering
    \includegraphics[width=\linewidth]{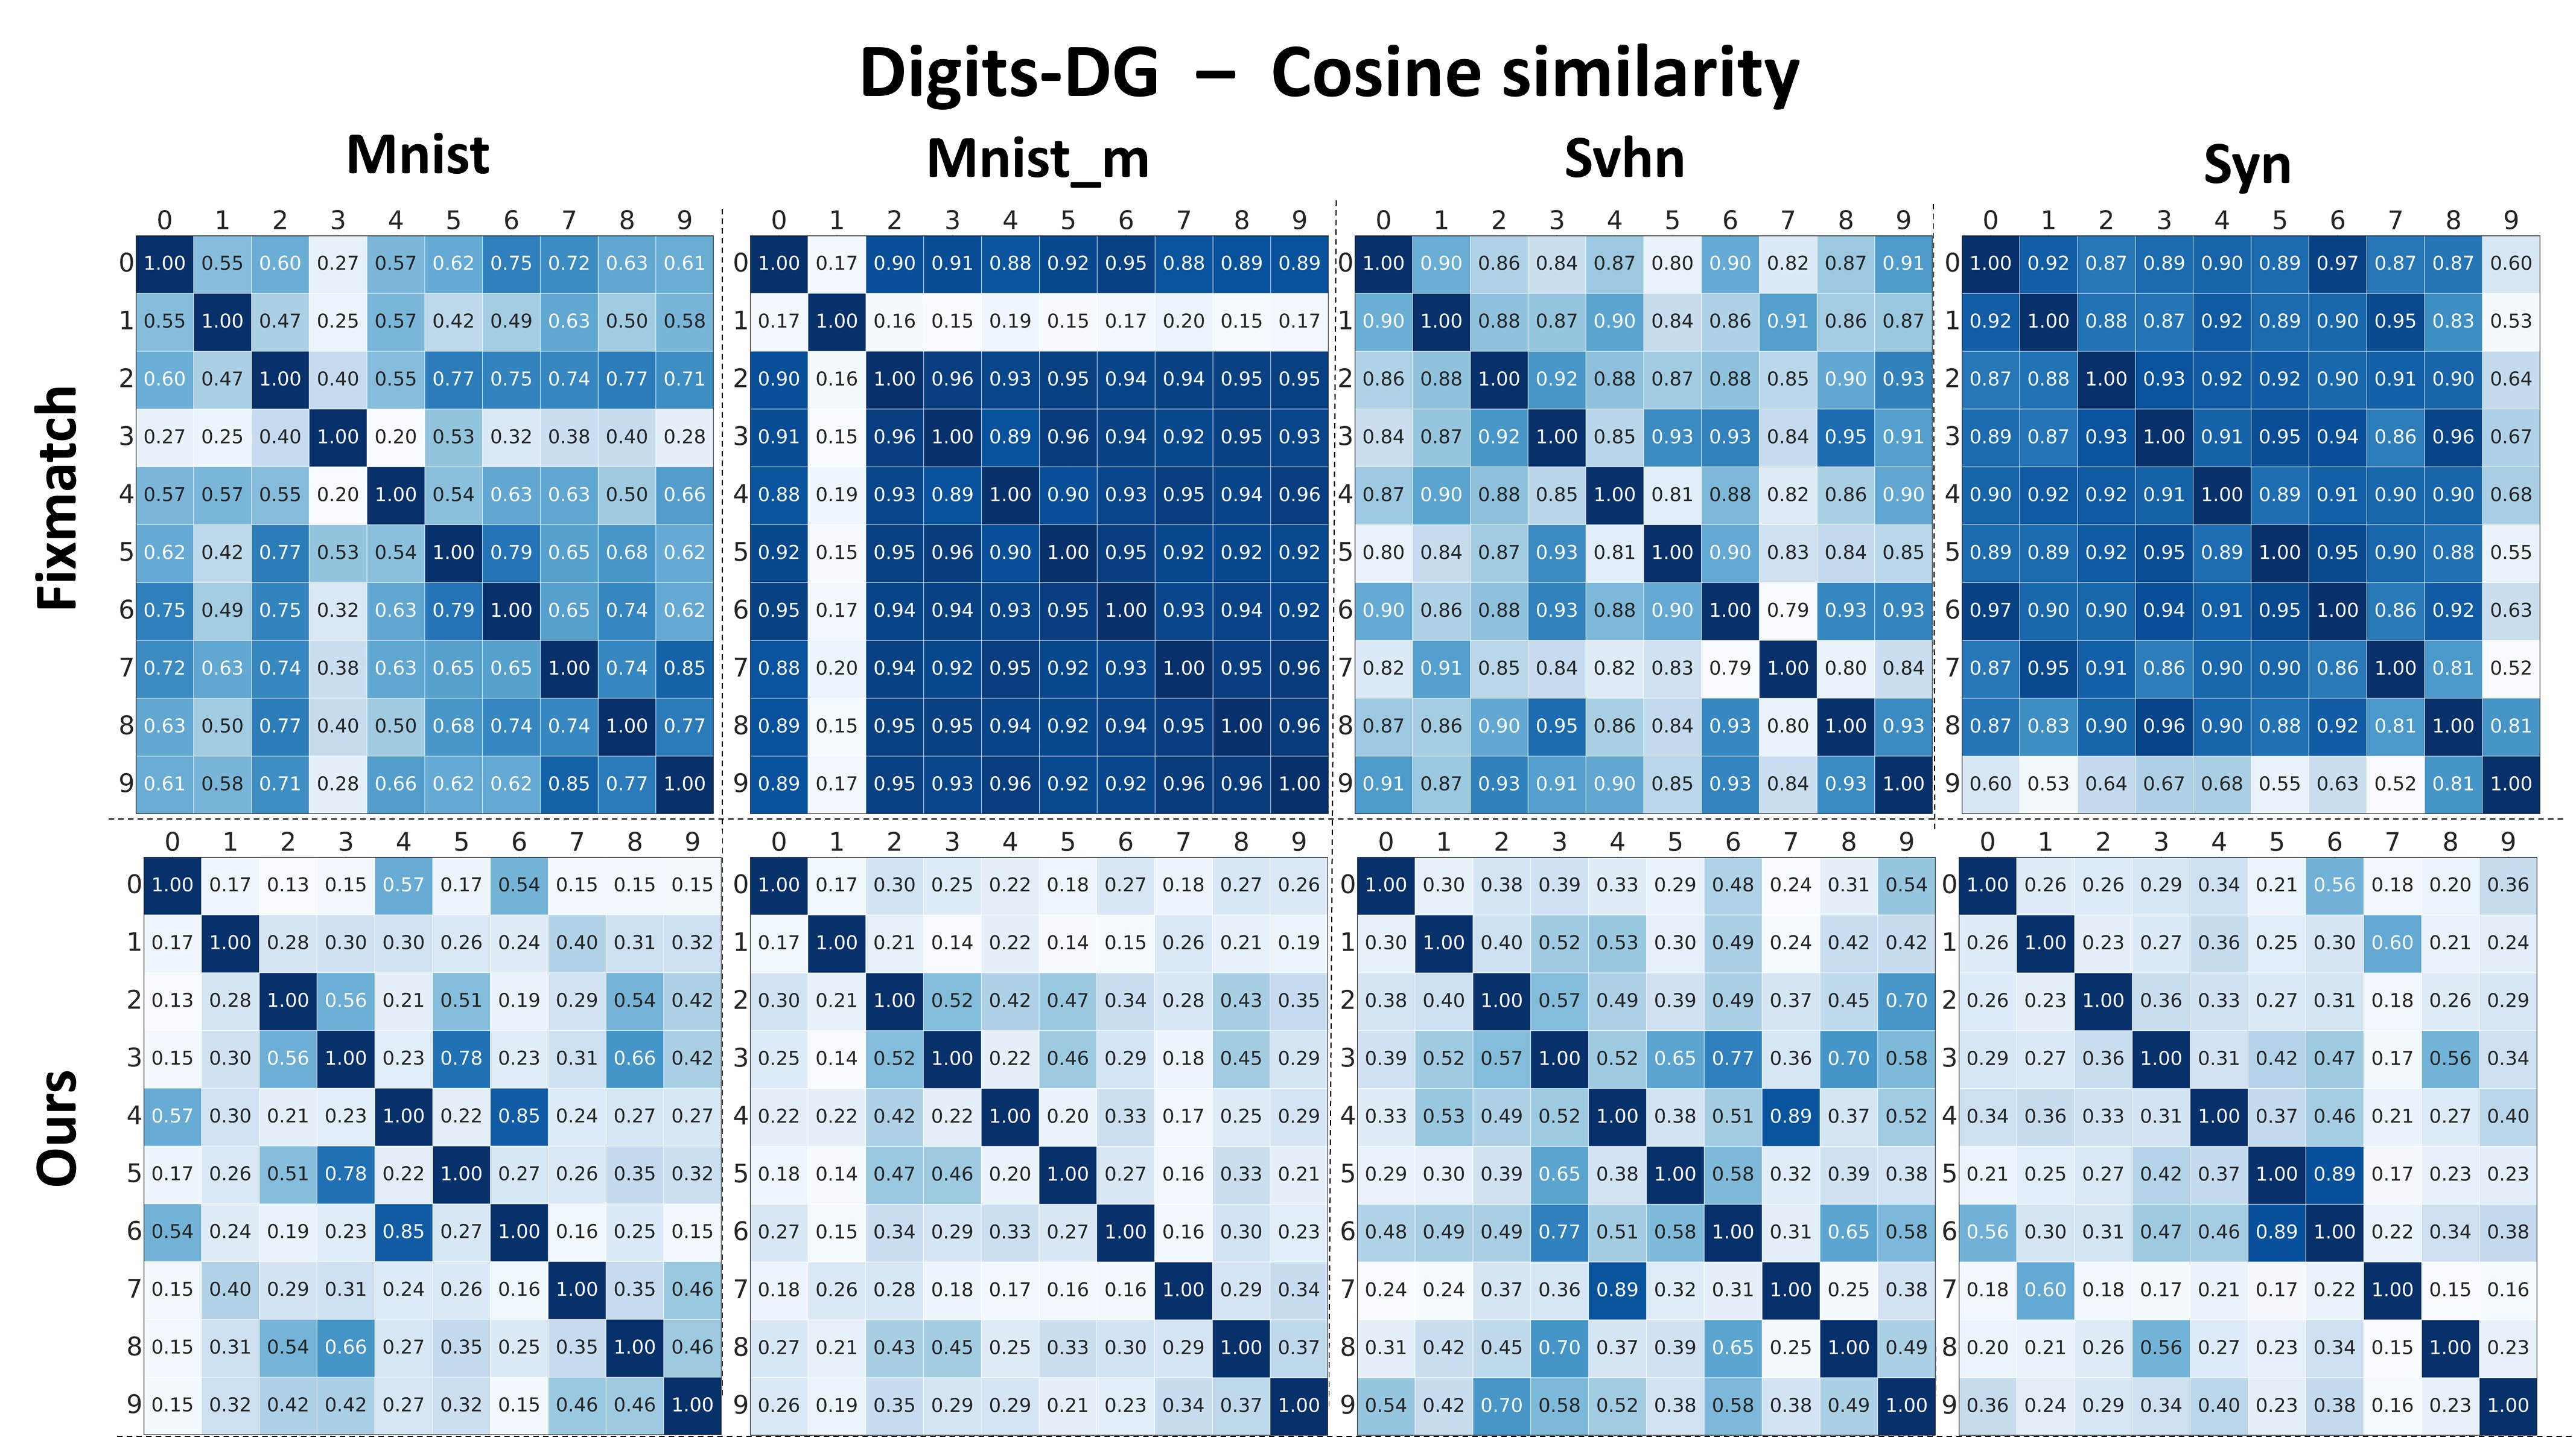}
    \caption{Comparison of cosine similarity of mean class features between Fixmatch and our method on Digits-DG.}
    \label{fig:Digits_sim}
\end{figure*}

\section{Confusion Matrices}

We plot the confusion matrices comparison between the Fixmatch baseline and our method on PACS (Fig.~\ref{fig:pacs_conf}), and Digits-DG (Fig.~\ref{fig:Digits_conf}) datasets. Compared to FixMatch, our approach shows improved class-wise accuracy in both datasets.

\begin{figure*}[!htp]
    \centering
    \includegraphics[width=\linewidth]{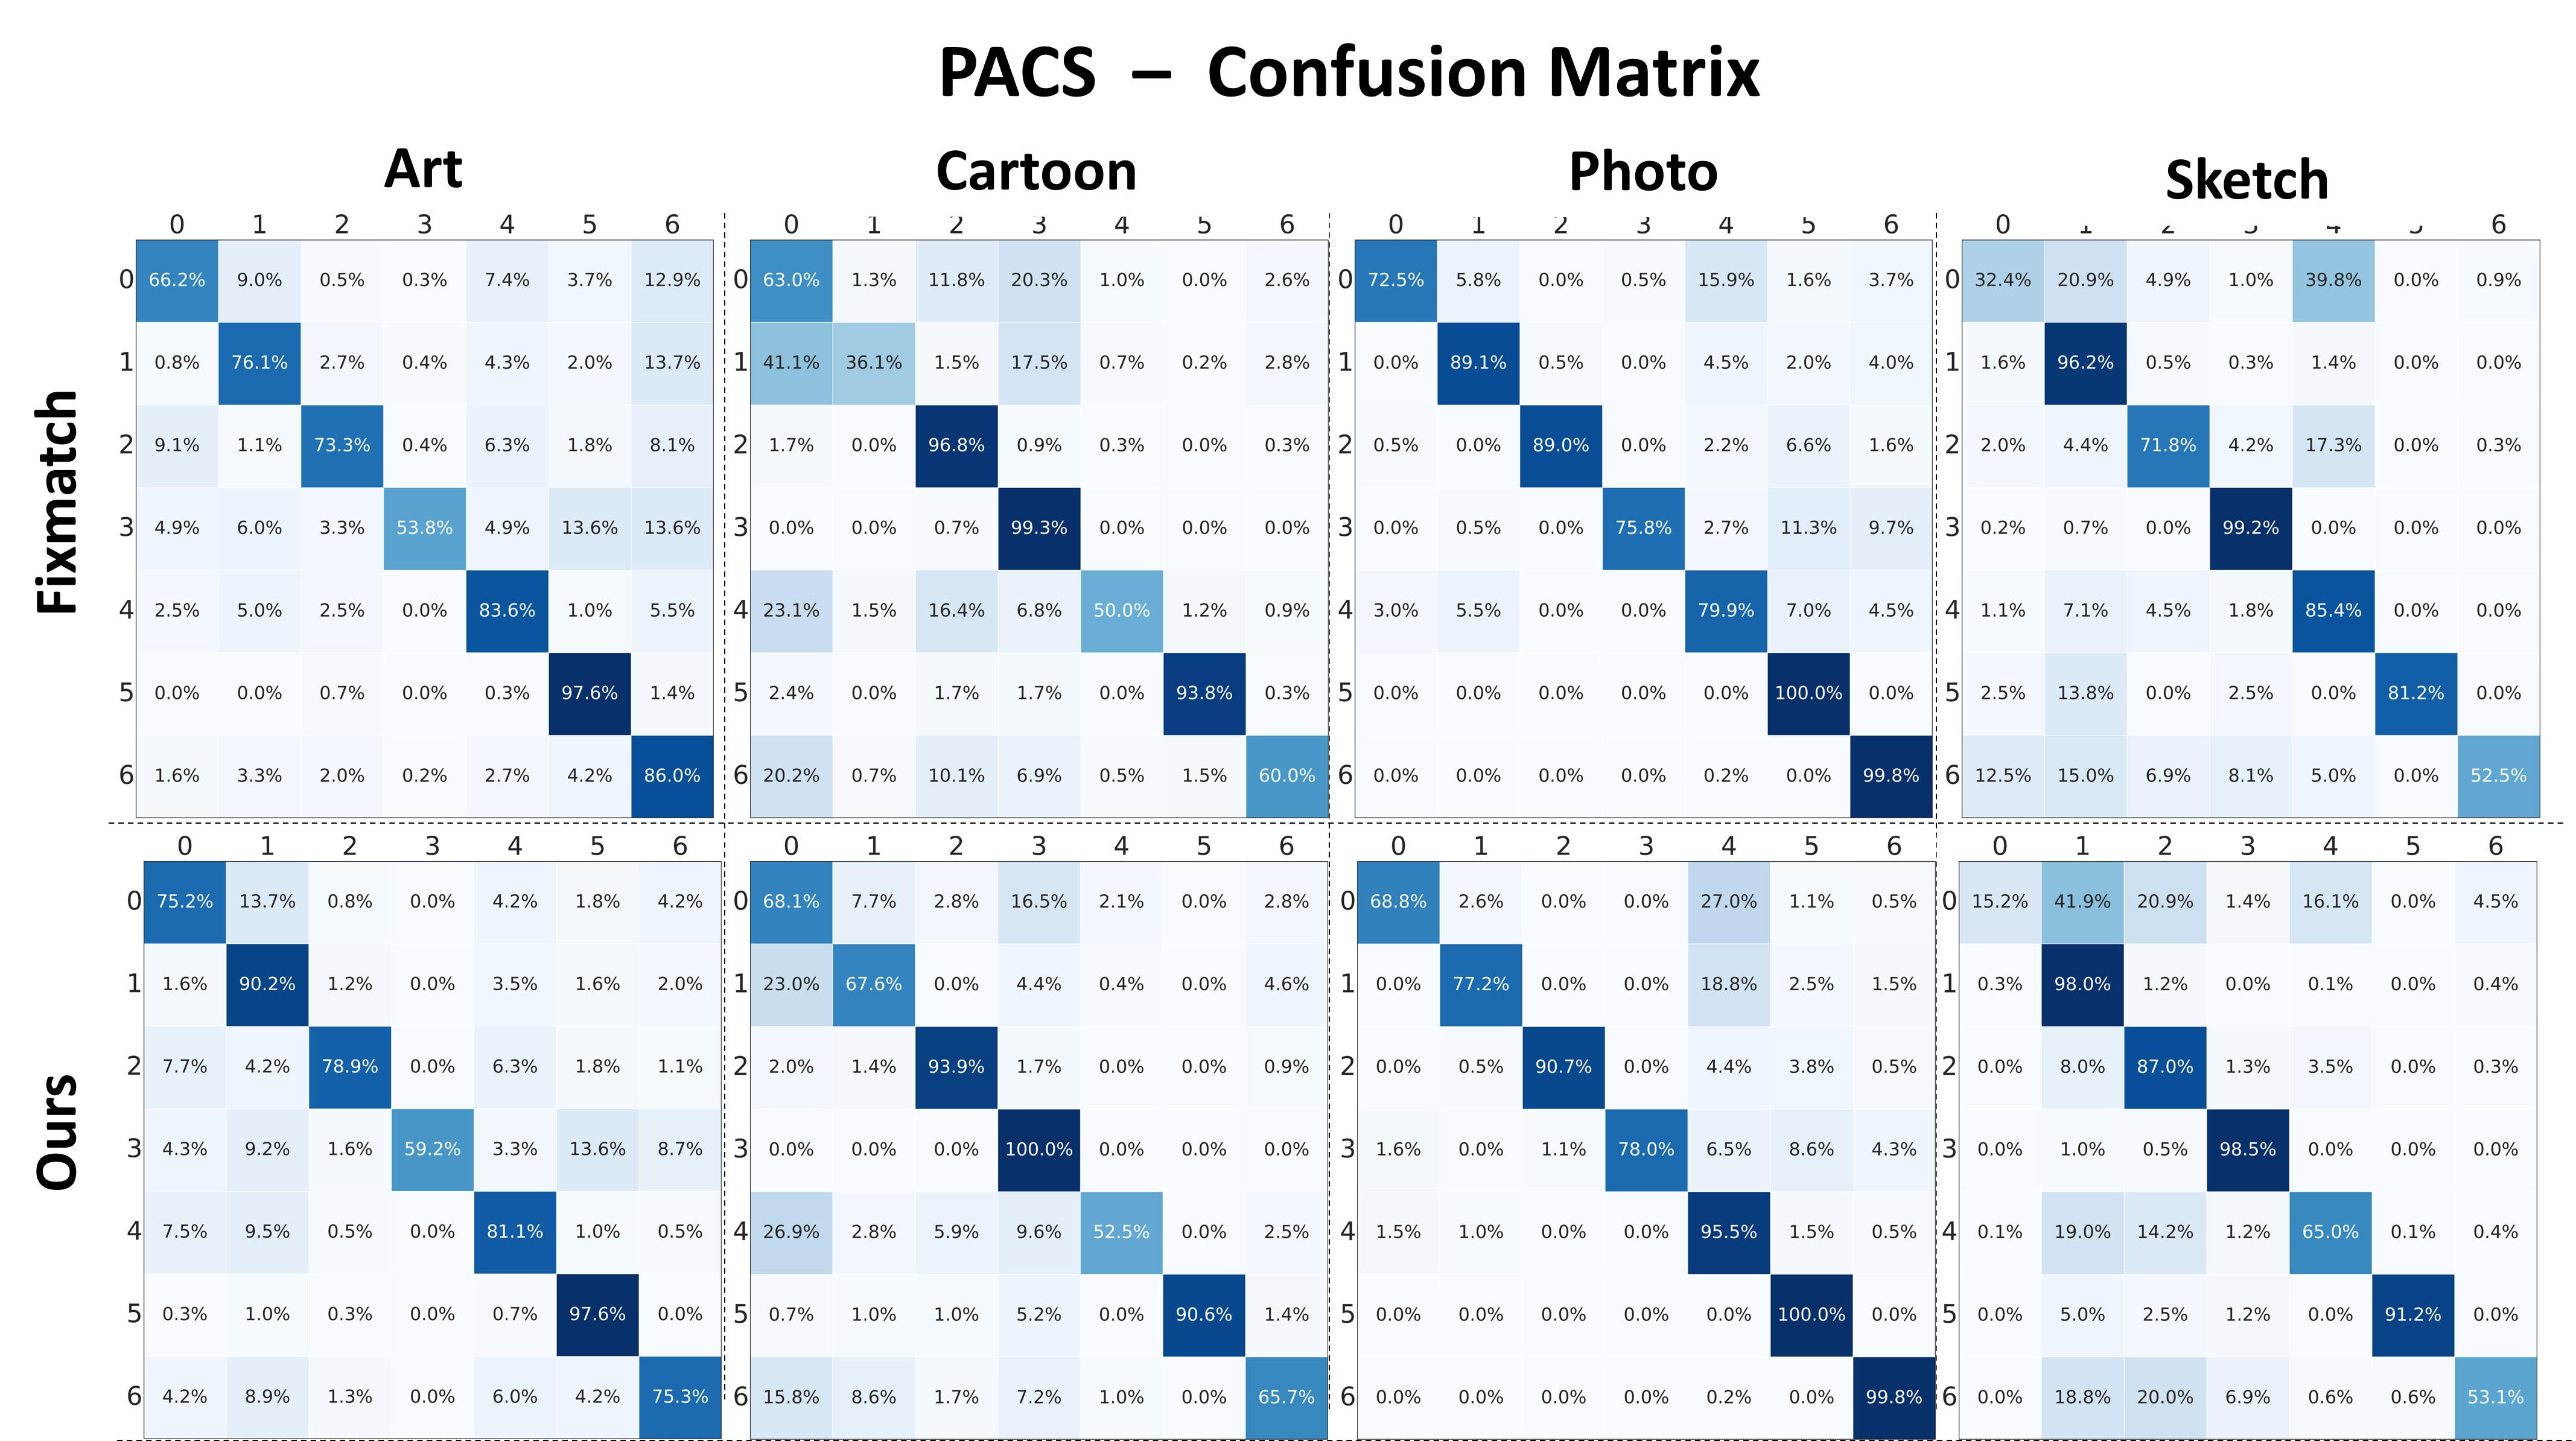}
    \caption{Confusion matrix comparison between Fixmatch and our method on PACS.}
    \label{fig:pacs_conf}
\end{figure*}

\begin{figure*}[!htp]
    \centering
    \includegraphics[width=\linewidth]{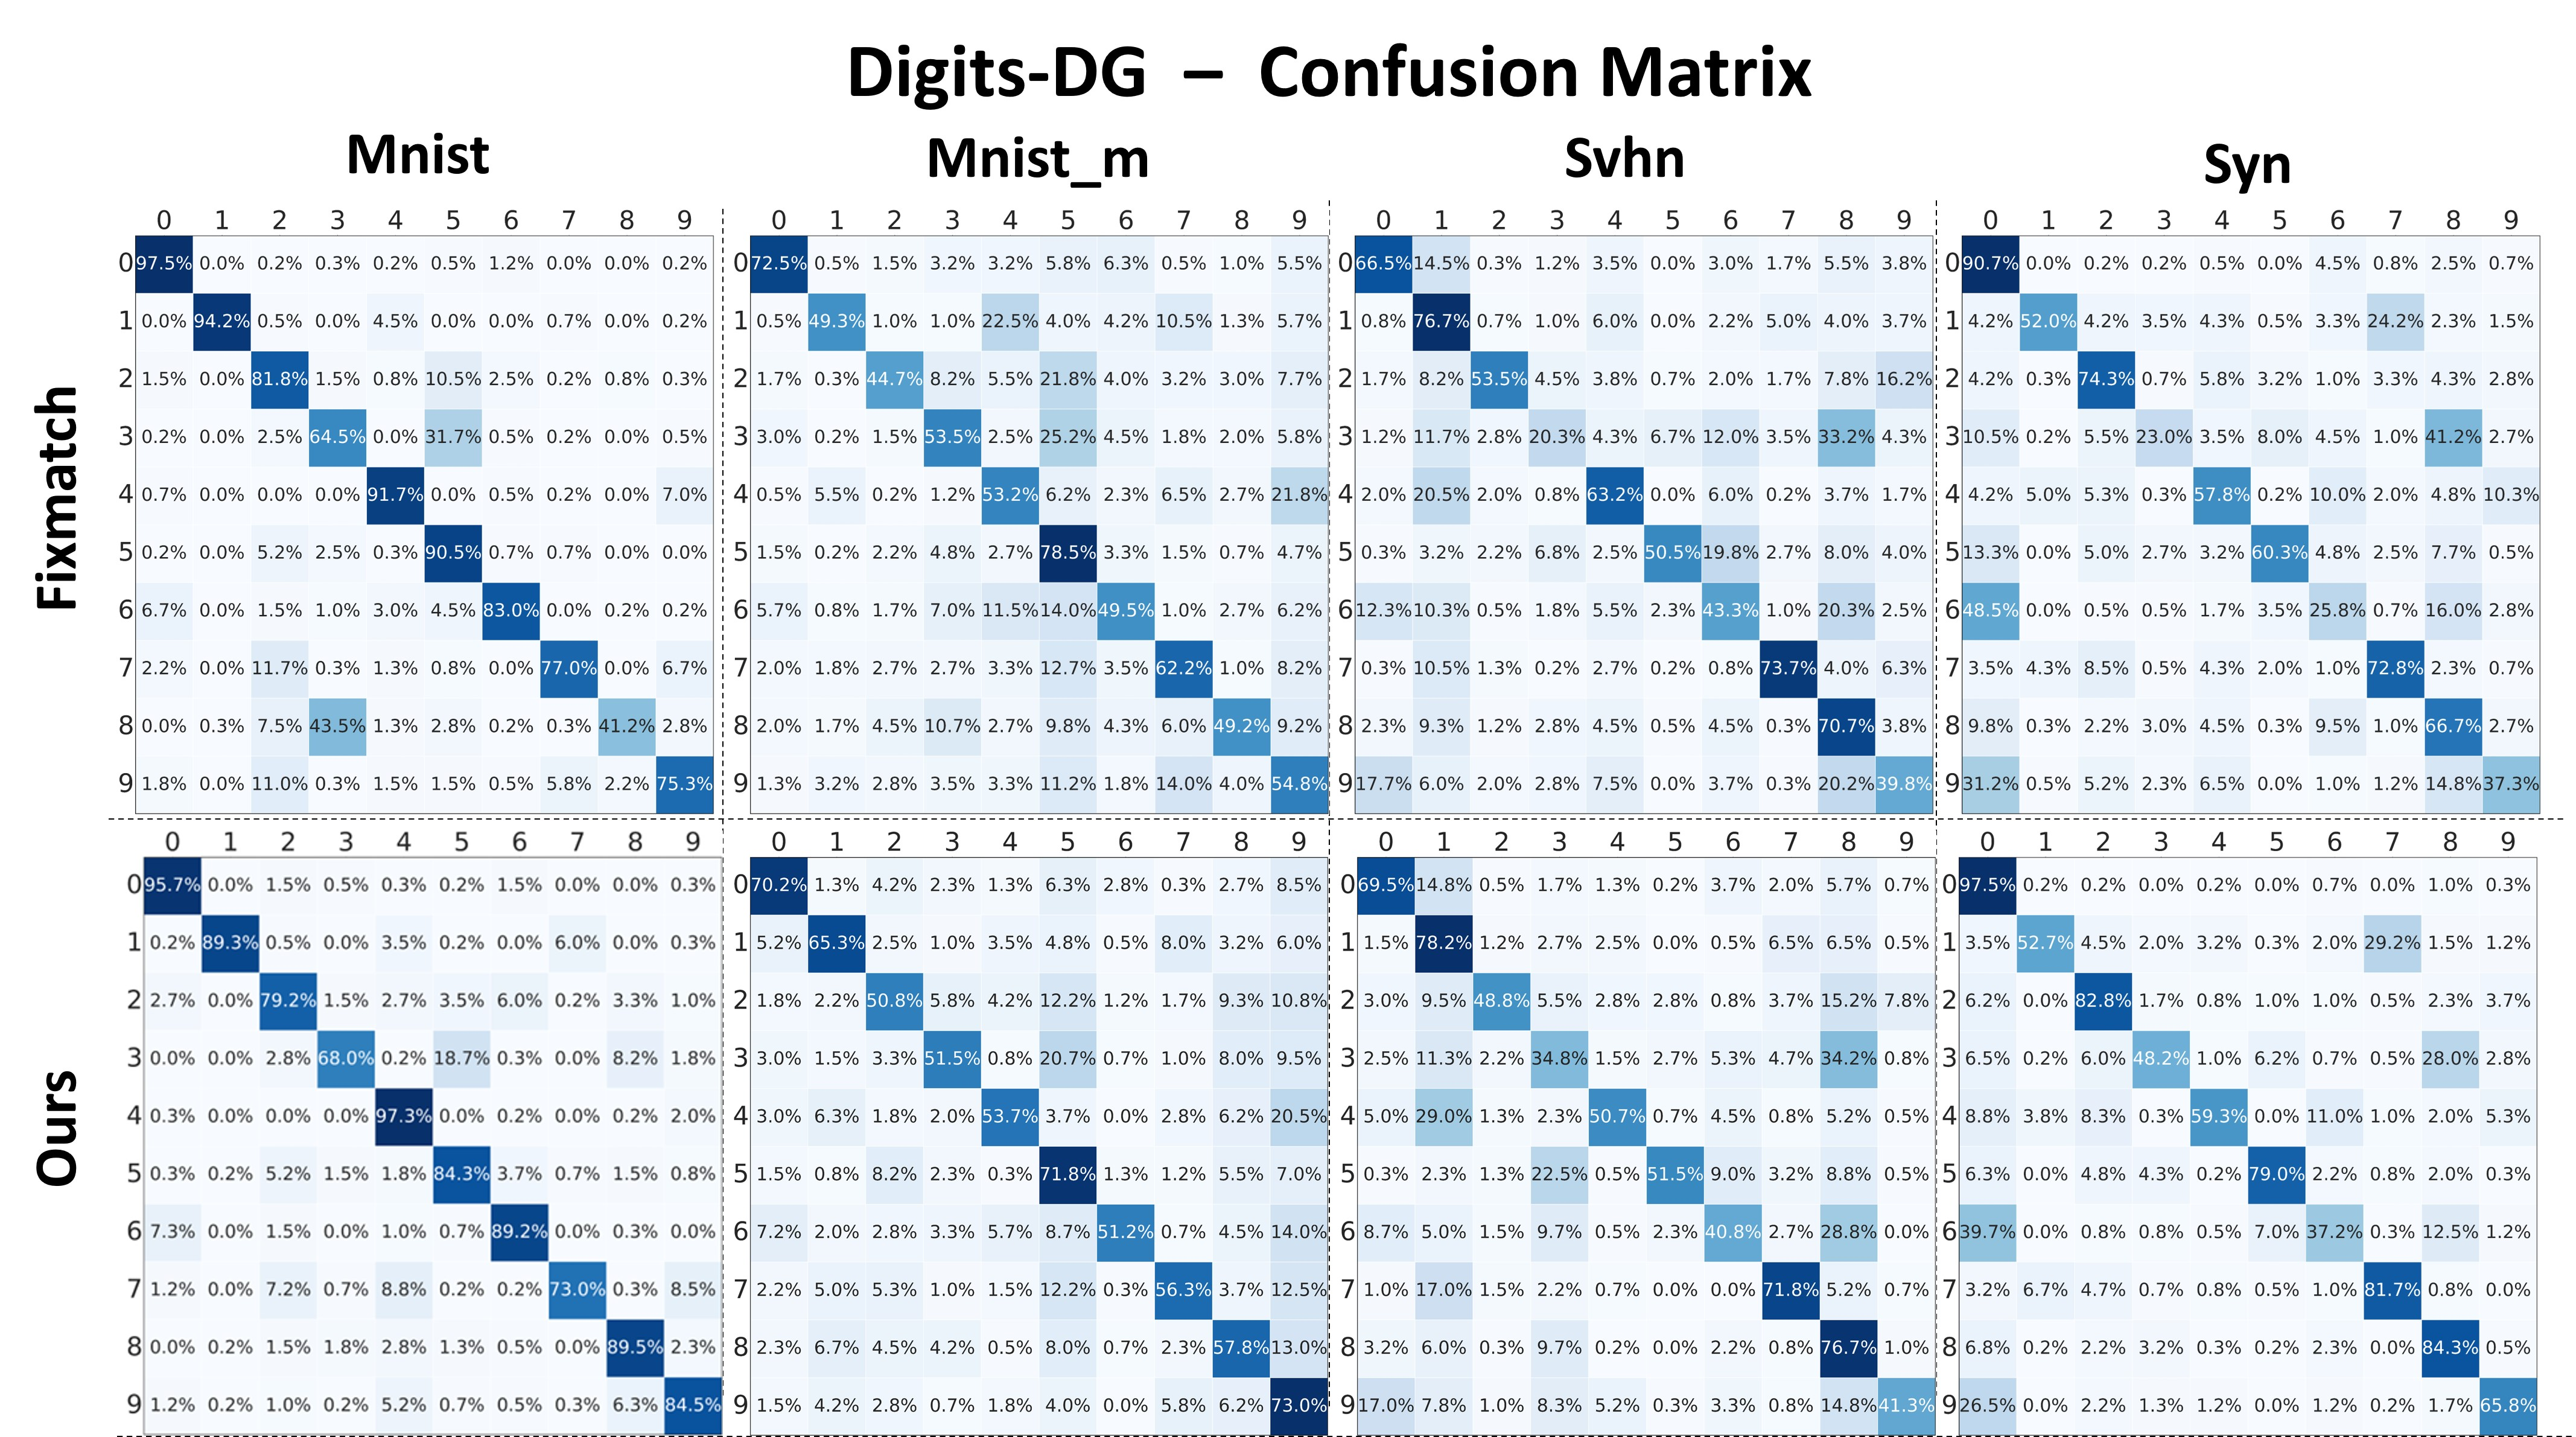}
    \caption{Confusion matrix for Fixmatch and our method on Digits-DG.}
    \label{fig:Digits_conf}
\end{figure*}

\section{Additional Feature Visualizations}

In addition to the feature visualization on PACS dataset (main manuscript), we visualize features on Digits-DG dataset in Fig.~\ref{fig:Digits_tsne} for Fixmatch and our method. In our approach, we observe that intra-class features are closer and inter-class features are far apart.  We note that, compared to the baseline, the classes are well-separated in our method. Also, the comparison of cosine similarity of mean class features in Fig.~\ref{fig:Digits_sim} validates this further.

\section{Comparison with other backbones}
For a fair comparison, we used the same backbone (ResNet18) as used in StyleMatch. To evaluate our method further, we analyze the performance OfficeHome dataset with several stronger backbones such as ImageNet pre-trained ResNet50, ResNet101, ViT-S/32, ViT-B/32, and CLIP pre-trained ViT-B/32 (CLIP-B/32) in Tab.~\ref{tab:other comparison}. Our method \emph{consistently outperforms} the baseline even with other stronger backbones. 

\section{Scaling of performance with \# labels}
Tab.~\ref{tab:scaling_labels} provides results with increasing number of per-class labels. We see that the performance of our method improves upon increasing the number of per-class labels and in all per-class labels settings, it is higher than the other methods. Furthermore, with just 100 per-class labels, our method performance is better than the fully supervised ERM (i.e. with all labels) that obtains \emph{80.0$_{\pm0.5}$}.

\section{Runtime and Memory overhead comparison}
To evaluate the effectiveness of our method, we compare the runtime and memory overhead (Tab.~\ref{tab:training time overhead comparison}.) Our method adds a little runtime overhead (20\%) over the baseline FixMatch compared to the existing SSDG method, StyleMatch (117\%) which has the same baseline (FixMatch).

\begin{table*}[!htp]
    \centering
    % \vspace{-0.8em}
        \begin{tabular}{lccccc}
            \toprule
            \textbf{Algorithm}  & \textbf{RN 50} & \textbf{RN 101} & \textbf{Vit-S/32} & \textbf{Vit-B/32} & \textbf{CLIP-B/32} \\
            \midrule
            FixMatch[32]            & 61.3$_{\pm0.4}$ & 62.8$_{\pm0.2}$ & 63.7$_{\pm0.5}$ & 72.0$_{\pm0.4}$ & 75.3$_{\pm0.6}$ \\
            FixM. +Ours       & \textbf{62.1$_{\pm0.4}$} & \textbf{64.2$_{\pm0.1}$} &\textbf{64.4$_{\pm0.3}$} & \textbf{72.9$_{\pm0.3}$} &\textbf{78.9$_{\pm0.4}$} \\
            \bottomrule
        \end{tabular}

    % \vspace{-1em}
    \caption{Results with different backbones on the Office Home dataset (10 labels per class)}
    % \vspace{-1.em}
    \label{tab:other comparison}
\end{table*}

\begin{table*}[!htp]
    \centering
 
    % \vspace{-0.95em}

        \begin{tabular}{lccccc}
            \toprule
            \textbf{Algorithm}  & \textbf{5} & \textbf{10} & \textbf{25} & \textbf{50} & \textbf{100} \\
            \midrule
            ERM[35]  & 51.2$_{\pm1.0}$ & 59.8$_{\pm2.5}$ & 66.7$_{\pm2.2}$ & 71.2$_{\pm1.9}$ & 75.7$_{\pm1.6}$ \\
            FixMatch[32]  & 72.8$_{\pm1.2}$ & 76.6$_{\pm1.2}$ & 77.6$_{\pm1.4}$ & 78.7$_{\pm0.4}$ & 79.4$_{\pm1.4}$ \\
            FixM.+Ours       & \textbf{77.3$_{\pm1.1}$} & \textbf{78.2$_{\pm1.2}$} & \textbf{79.3$_{\pm1.8}$} & \textbf{79.6$_{\pm1.0}$} & \textbf{80.4$_{\pm0.6}$} \\
            \bottomrule
        \end{tabular}

    % \vspace{-1em}
    \caption{Results with different per class labels on PACS}
    % \vspace{-1.em}
    \label{tab:scaling_labels}
\end{table*}

\begin{table*}[!htp]
    \centering
 
    \small
    % \vspace{-0.95em}

    \begin{tabular}{lcccc}
\toprule
 \textbf{Algorithm}                      & \textbf{s/epoch}    & \textbf{Overhead}  & \textbf{GPU Mem(MB)}    & \textbf{Overhead}    \\
\midrule
FixMatch[32] & 44.4           & -    & 5595 & -  \\
StyleMatch[57]  & 96.38           & +117.07 \%   & 7561 & +35.13 \% \\
FixM.+Ours  & 52.85           & +20.11 \% & 7647 & +36.67 \%    \\
\bottomrule
\end{tabular}
    % \vspace{-1em}
    \caption{Runtime (s/epoch) and memory (MB) overhead  }
    \label{tab:training time overhead comparison}
    % \vspace{-1.em}
\end{table*}

% \begin{figure*}[!htp]
% % \vspace{-1em}
%     \centering
%     \includegraphics[width=\linewidth]{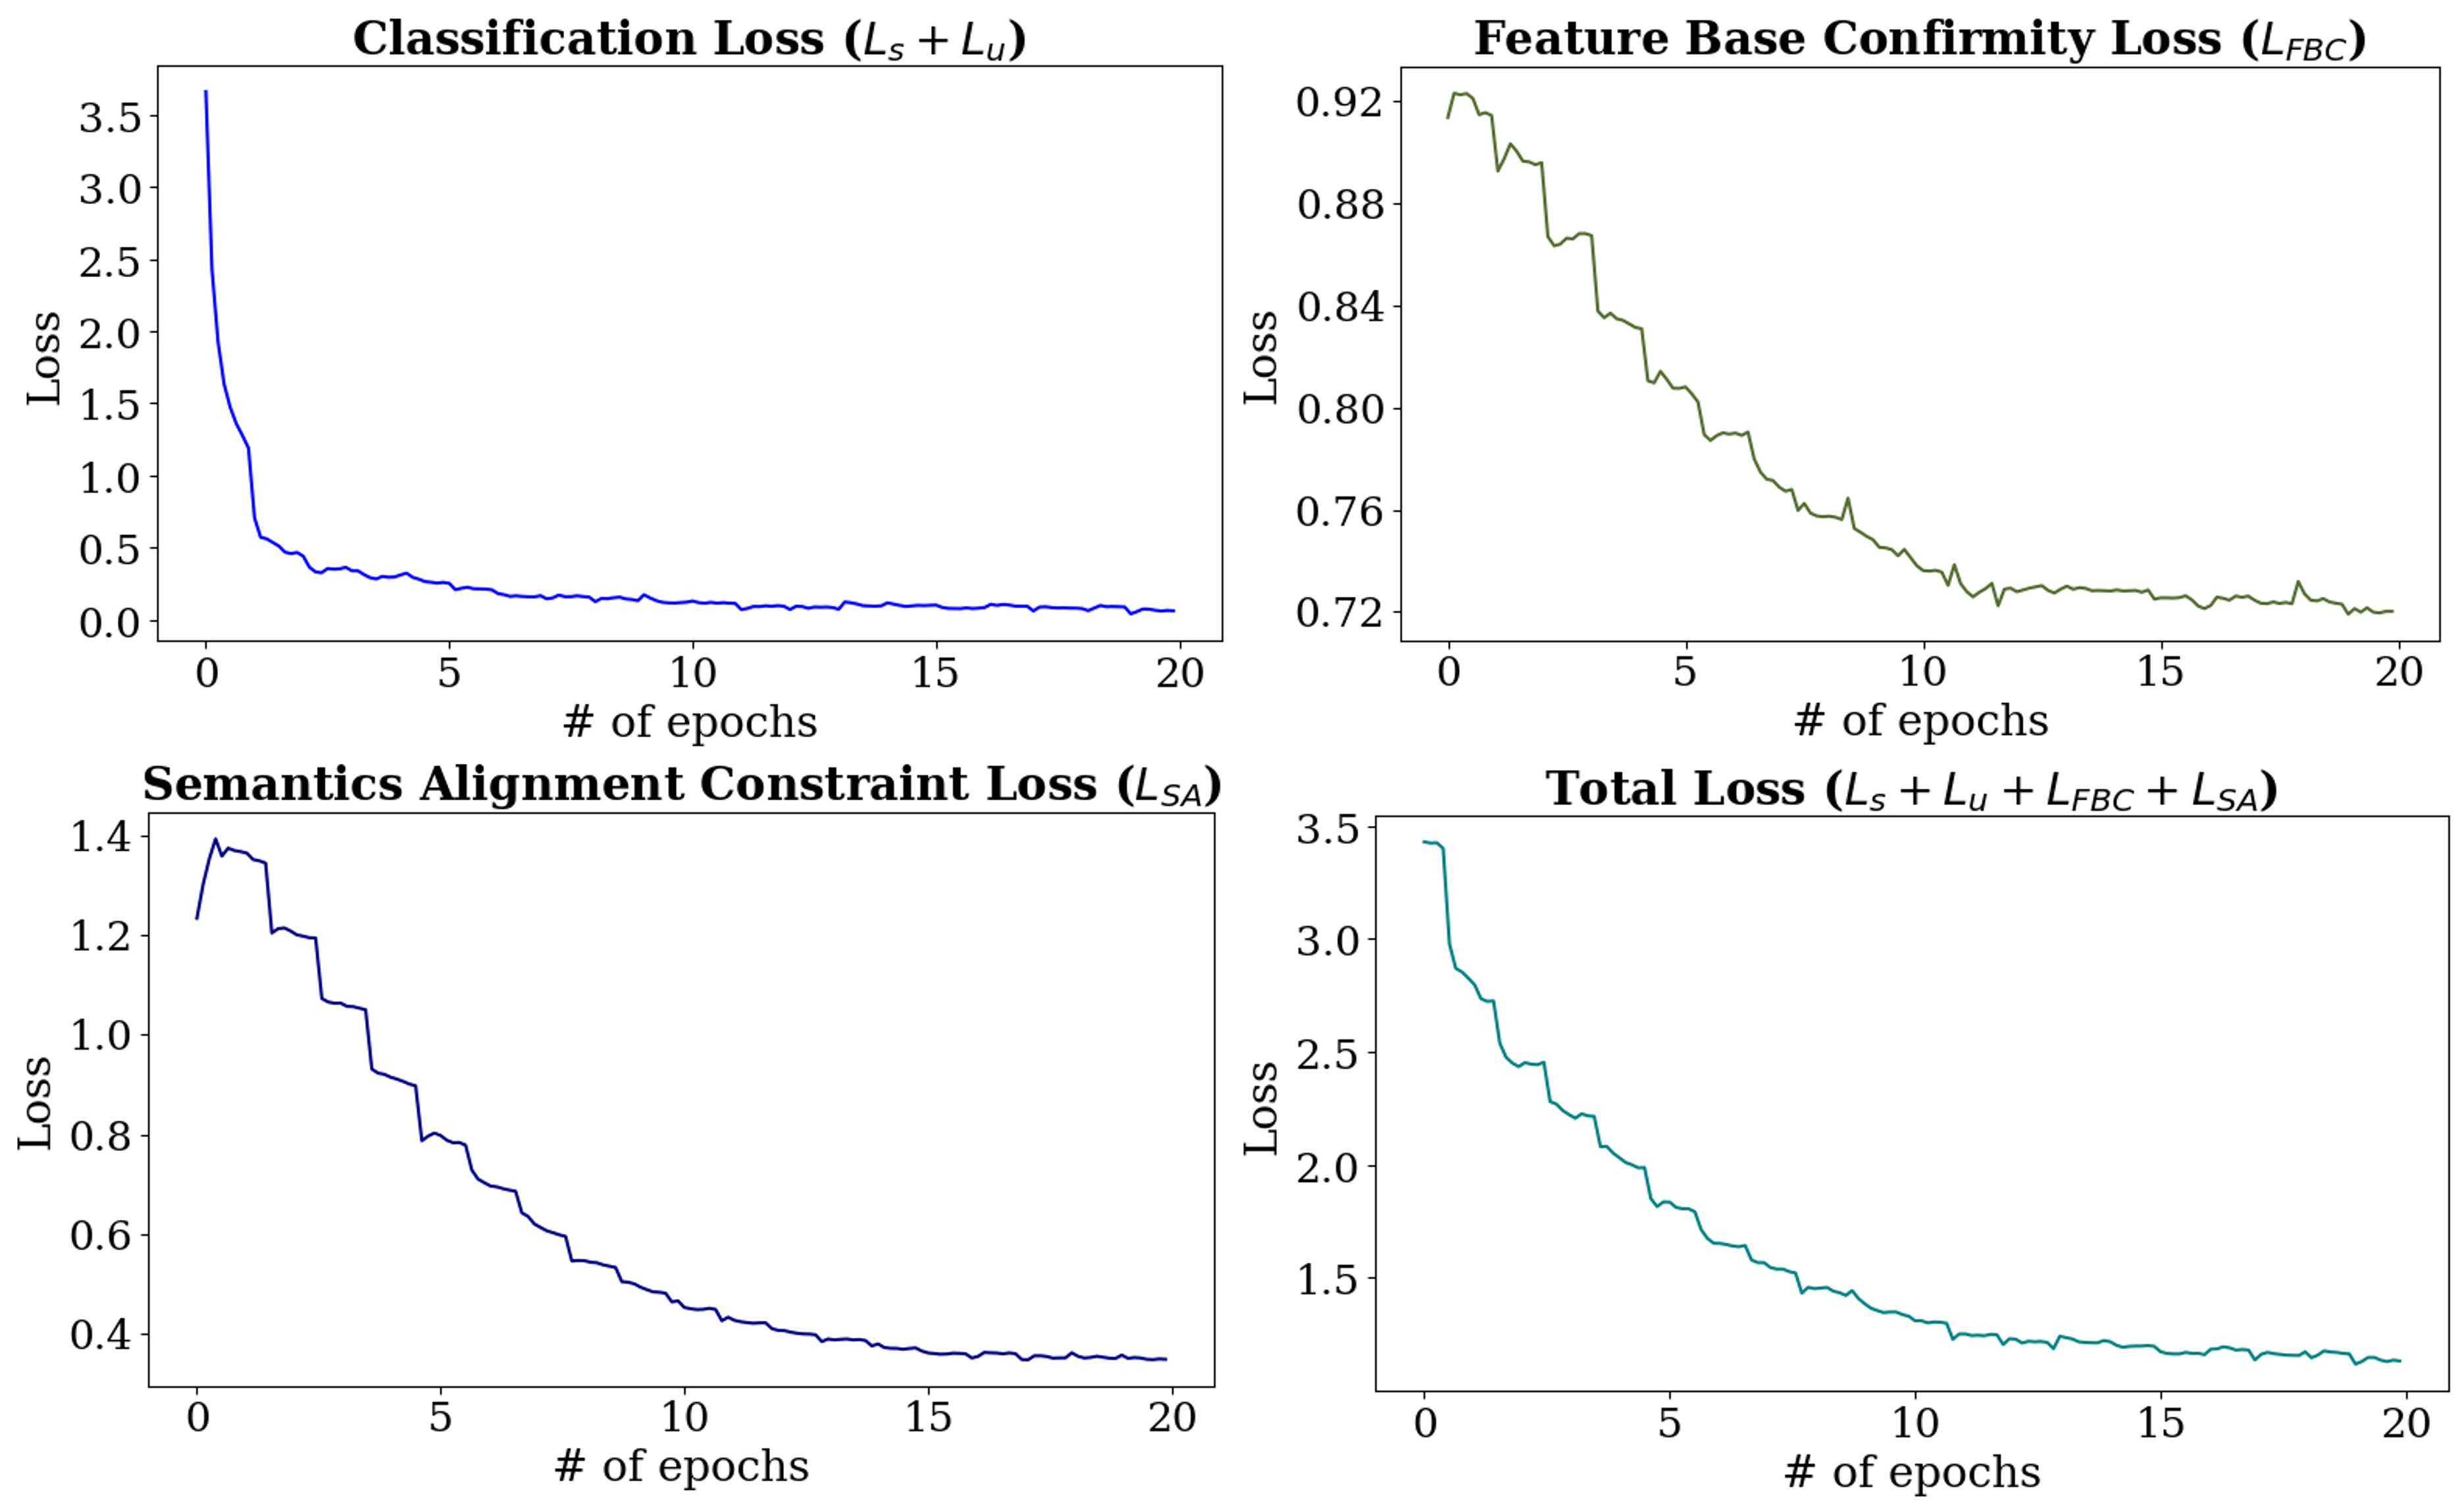}
%     % \vspace{-2em}
%     \caption{Loss curves during training}
%     % \vspace{-1em}
%     \label{fig:loss-curves}
%     % \vspace{-2em}
% \end{figure*}

\begin{figure*}[!htp]
    \centering
    \includegraphics[width=\linewidth]{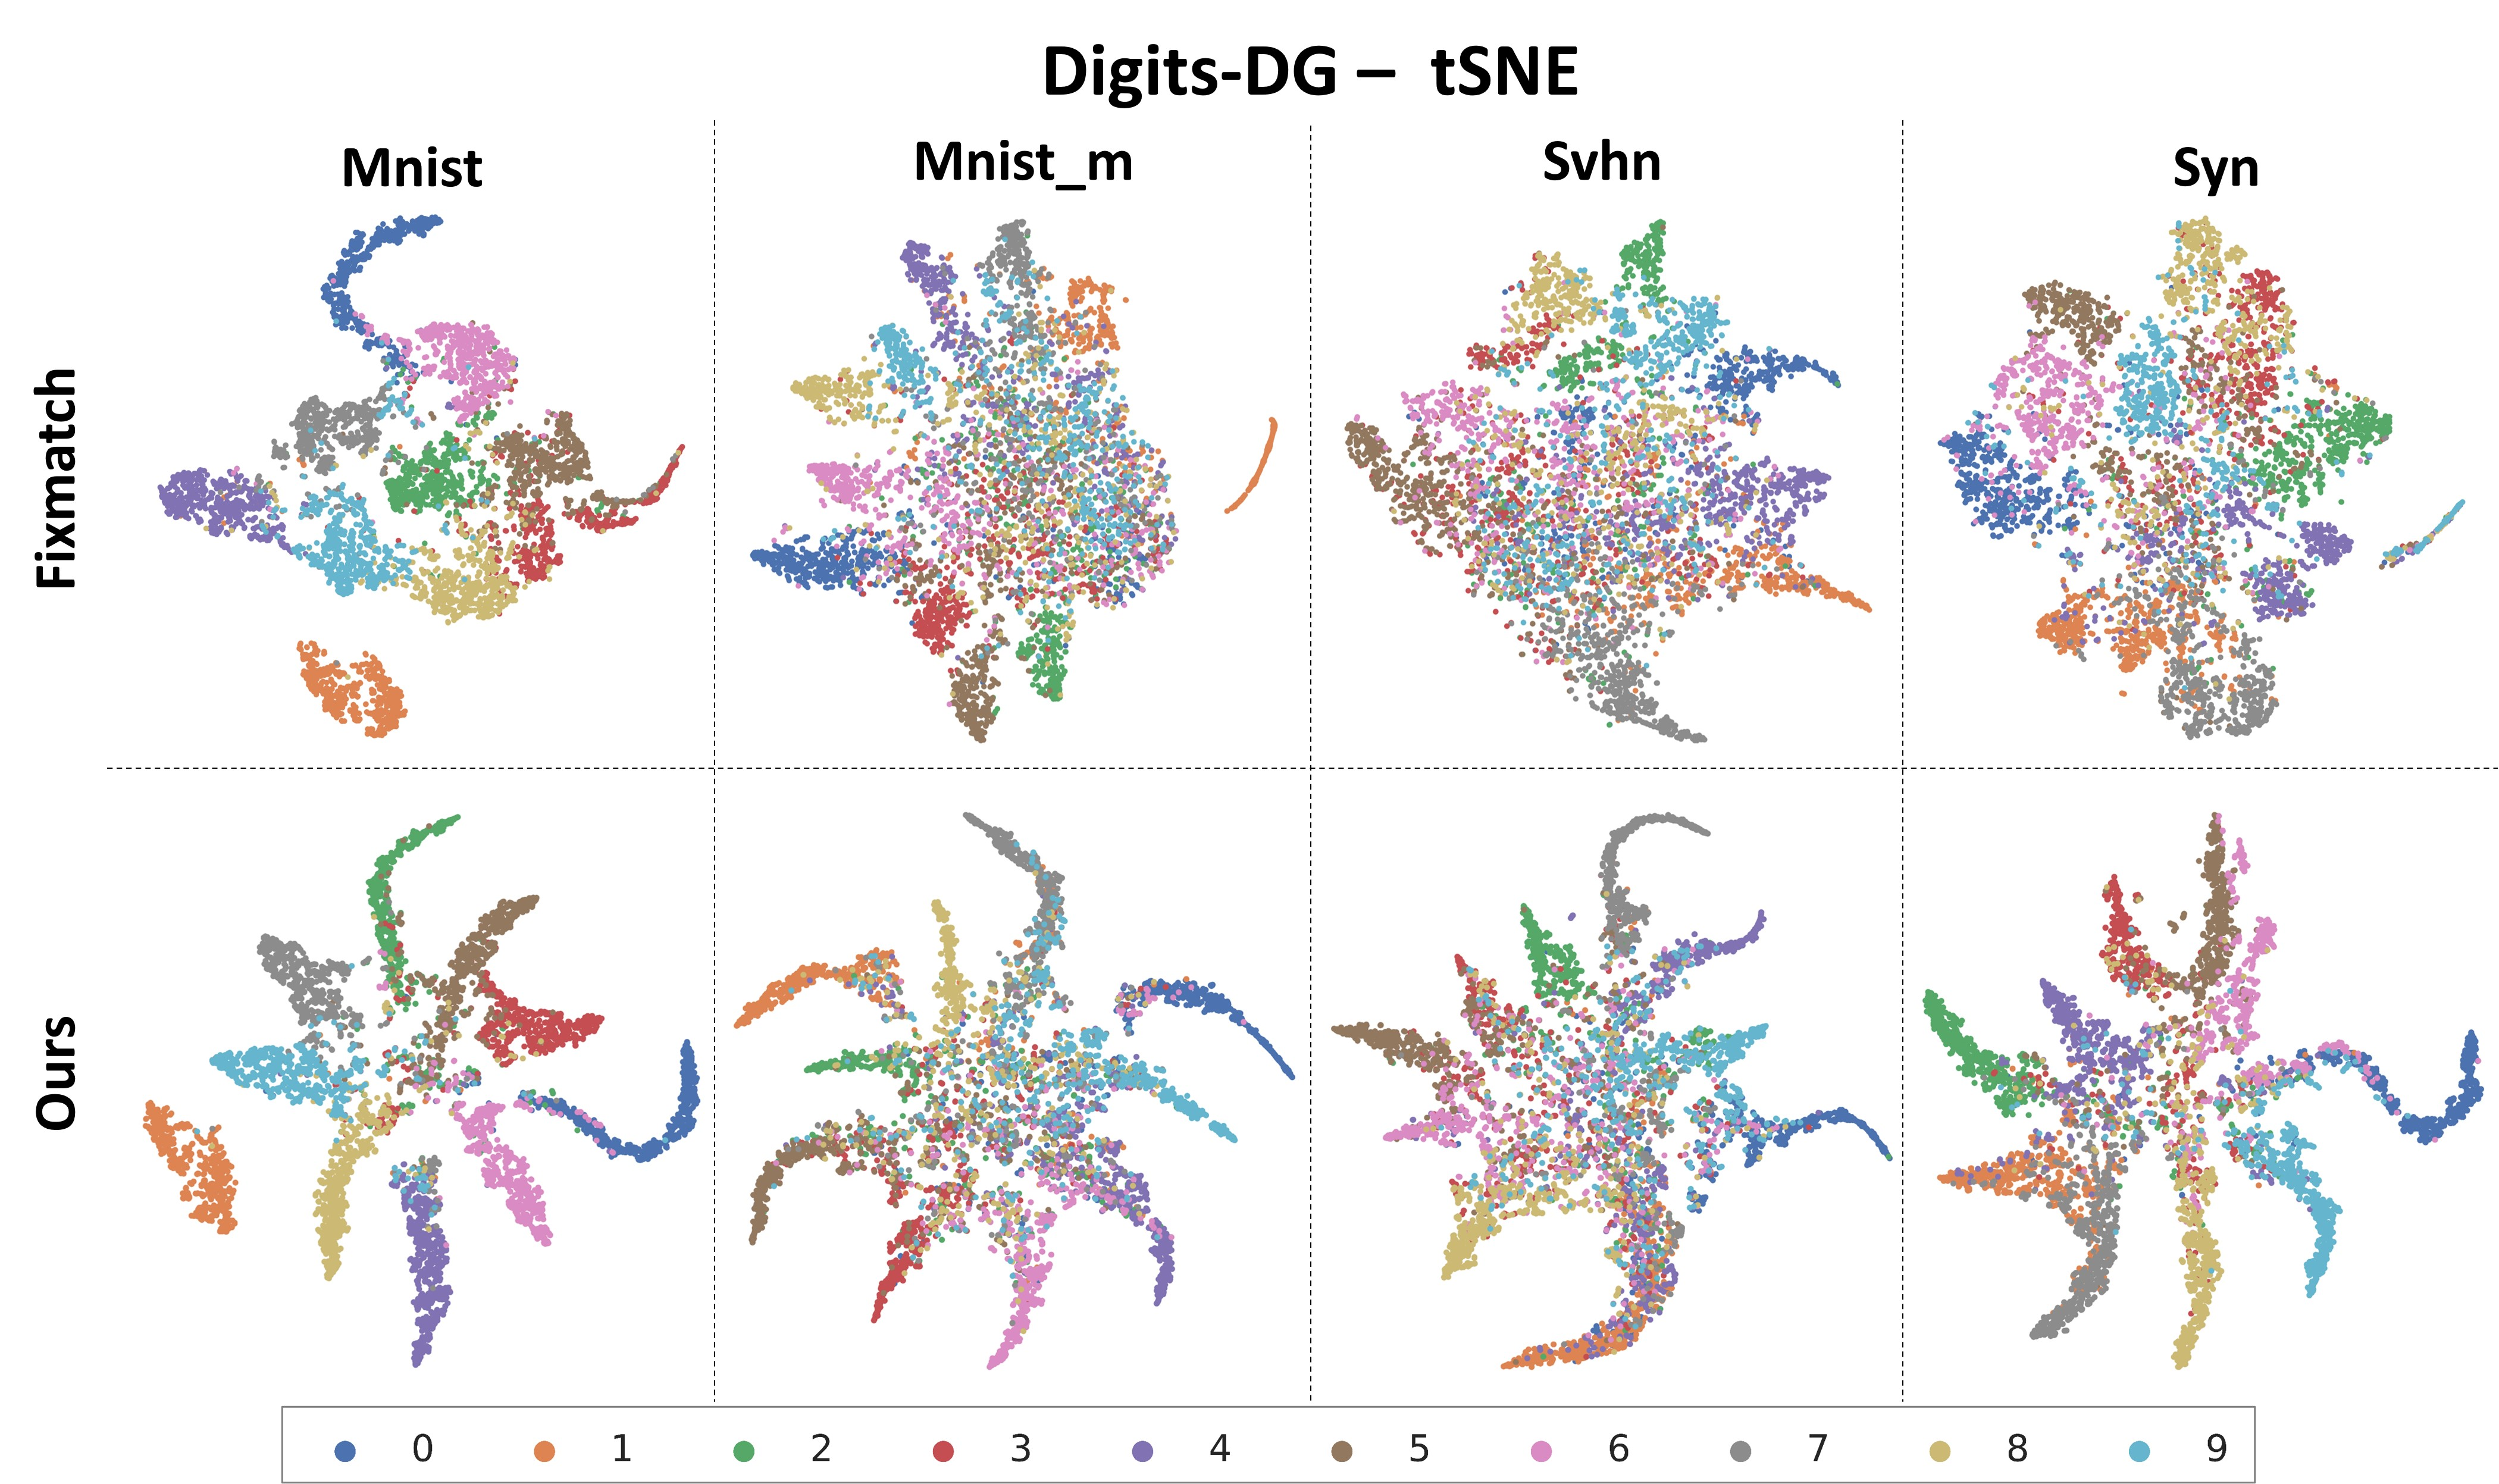}
    \caption{Feature visualization using tSNE for Fixmatch and ours on Digits-DG. Our method facilitates learning more discriminative features under various domain shifts and limited labels.}
    \label{fig:Digits_tsne}
\end{figure*}
